# Supplementary material for: Evanescent Operators in One-Loop Matching Computations
Source: arXiv:2211.09144 ancillary file (2023-02-08)
Supplement: Supplementary file 1 [file resulttable.pdf]

# Evanescent Operators in One-Loop Matching Computations

---

Javier Fuentes-Martín,<sup>1,2\*</sup> Matthias König,<sup>3†</sup> Julie Pagès,<sup>4‡</sup>  
Anders Eller Thomsen,<sup>5§</sup> and Felix Wilsch<sup>6¶</sup>

<sup>1</sup> Departamento de Física Teórica y del Cosmos, Universidad de Granada,  
Campus de Fuentenueva, E-18071 Granada, Spain,

<sup>2</sup> PRISMA Cluster of Excellence & Mainz Institute for Theoretical Physics,  
Johannes Gutenberg University, D-55099 Mainz, Germany,

<sup>3</sup> Physik Department T31, Technische Universität München,  
James-Franck-Str. 1, D-85748 Garching, Germany

<sup>4</sup> Department of Physics, University of California at San Diego,  
9500 Gilman Drive, La Jolla, CA 92093-0319, USA

<sup>5</sup> Albert Einstein Center for Fundamental Physics, Institute for Theoretical Physics,  
University of Bern, CH-3012 Bern, Switzerland

<sup>6</sup> Physik-Institut, Universität Zürich, CH-8057 Zürich, Switzerland

*January 19, 2023*

---

\*javier.fuentes@ugr.es

†matthias.koenig@tum.de

‡julie.pages@physics.ucsd.edu

§thomsen@itp.unibe.ch

¶felix.wilsch@physik.uzh.ch

# 1 Notation and Conventions

We list the redundant operators  $R$  in Table 1. For the SM Lagrangian we use the following notation:

$$\begin{aligned} \mathcal{L}_{\text{SM}} = & -\frac{1}{4}G_{\mu\nu}^A G^{\mu\nu A} - \frac{1}{4}W_{\mu\nu}^I W^{\mu\nu I} - \frac{1}{4}B_{\mu\nu} B^{\mu\nu} + (D_\mu H)^\dagger (D^\mu H) + \mu^2 (H^\dagger H) - \frac{\lambda}{2} (H^\dagger H)^2 \\ & + \sum_{\psi=q,u,d,\ell,e} \bar{\psi} i \not{D} \psi - \left( y_u^{pr} \bar{q}_p \tilde{H} u_r + y_d^{pr} \bar{q}_p H d_r + y_e^{pr} \bar{\ell}_p H e_r + \text{h.c.} \right), \end{aligned} \quad (1.1)$$

where we keep the gauge-fixing and ghost Lagrangians implicit. The matter content is defined as usual, with  $p$  and  $r$  denoting flavor indices. The conjugated Higgs doublet is given by  $\tilde{H}^i = \varepsilon^{ij} H_j^*$ , where  $\varepsilon^{ij}$  is the anti-symmetric SU(2) invariant tensor defined by  $\varepsilon^{12} = +1$  and  $\varepsilon^{ij} = -\varepsilon^{ji}$ . The covariant derivative is defined as

$$D_\mu = \partial_\mu - i g_s T^A G_\mu^A - i g_L t^I W_\mu^I - i g_Y Y B_\mu, \quad (1.2)$$

where the SU(3)<sub>c</sub> and SU(2)<sub>L</sub> generators are given by  $T^A = \lambda^A/2$  and  $t^I = \tau^I/2$ , respectively, with  $\lambda^A$  being the Gell-Mann matrices and  $\tau^I$  the Pauli matrices. For the  $U(1)_Y$  hypercharge,  $Y$ , we use the convention

$$\begin{aligned} Y_q &= \frac{1}{6}, & Y_u &= \frac{2}{3}, & Y_d &= -\frac{1}{3}, \\ Y_\ell &= -\frac{1}{2}, & Y_e &= -1, & Y_H &= \frac{1}{2}. \end{aligned} \quad (1.3)$$

The corresponding gauge couplings are dubbed  $g_s$ ,  $g_L$ , and  $g_Y$ , respectively. The field strength tensors read

$$\begin{aligned} G_{\mu\nu}^A &= \partial_\mu G_\nu^A - \partial_\nu G_\mu^A + g_s f_{ABC} G_\mu^B G_\nu^C, \\ W_{\mu\nu}^I &= \partial_\mu W_\nu^I - \partial_\nu W_\mu^I + g_L \varepsilon_{IJK} W_\mu^J W_\nu^K, \\ B_{\mu\nu} &= \partial_\mu B_\nu - \partial_\nu B_\mu, \end{aligned} \quad (1.4)$$

where  $f_{ABC}$  and  $\varepsilon_{IJK}$  are the SU(3)<sub>c</sub> and SU(2)<sub>L</sub> structure constants, respectively. For the SMEFT operators we use the same definitions as in [1], but with dual tensors,  $\tilde{X}^{\mu\nu} = \frac{1}{2} \varepsilon^{\mu\nu\rho\sigma} X_{\rho\sigma}$ , following the  $\varepsilon^{0123} = +1$  convention.

In the results below we use the following short-hand notation for the Yukawa interactions and Higgs potential terms:

$$Q_{yu}^{pr} = \bar{q}_p \tilde{H} u_r, \quad Q_{yd}^{pr} = \bar{q}_p H d_r, \quad Q_{ye}^{pr} = \bar{\ell}_p H e_r, \quad Q_\mu = H^\dagger H, \quad Q_\lambda = (H^\dagger H)^2. \quad (1.5)$$

In expressions where there is a reading point ambiguity, we encode it using the parameter  $\xi_{\text{rp}}$ . See Section 2.2 of the paper for more details. Furthermore, complex conjugation for couplings and operators is denoted with a bar, *e.g.* for the case of one of the operators

$$Q_{\ell equ}^{(1)ptsr} = (\bar{\ell}_{ip} e_t) \varepsilon^{ij} (\bar{q}_{js} u_r), \quad \overline{Q_{\ell equ}^{(1)ptsr}} = (\bar{e}_t \ell_{ip}) \varepsilon^{ij} (\bar{u}_r q_{js}). \quad (1.6)$$

| Scalar currents                                         |                                                                                  |                              |                                                                                                                                        |
|---------------------------------------------------------|----------------------------------------------------------------------------------|------------------------------|----------------------------------------------------------------------------------------------------------------------------------------|
| $(\bar{L}R)(\bar{R}L) \text{ \& } (\bar{L}R)(\bar{L}R)$ |                                                                                  | $(\bar{R}^c R)(\bar{R}R^c)$  |                                                                                                                                        |
| $R_{\ell e}$                                            | $(\bar{\ell}_p e_r)(\bar{e}_s \ell_t)$                                           | $R_{e^c e}$                  | $(\bar{e}_p^c e_r)(\bar{e}_s e_t^c)$                                                                                                   |
| $R_{\ell u}$                                            | $(\bar{\ell}_p u_r)(\bar{u}_s \ell_t)$                                           | $R_{u^c u}$                  | $(\bar{u}_{\alpha p}^c u_{\beta r})(\bar{u}_{\beta s} u_{\alpha t}^c)$                                                                 |
| $R_{\ell d}$                                            | $(\bar{\ell}_p d_r)(\bar{d}_s \ell_t)$                                           | $R_{d^c d}$                  | $(\bar{d}_{\alpha p}^c d_{\beta r})(\bar{d}_{\beta s} d_{\alpha t}^c)$                                                                 |
| $R_{qe}$                                                | $(\bar{q}_p e_r)(\bar{e}_s q_t)$                                                 | $R_{e^c u}$                  | $(\bar{e}_p^c u_r)(\bar{u}_s e_t^c)$                                                                                                   |
| $R_{qu}^{(1)}$                                          | $(\bar{q}_p u_r)(\bar{u}_s q_t)$                                                 | $R_{e^c d}$                  | $(\bar{e}_p^c d_r)(\bar{d}_s e_t^c)$                                                                                                   |
| $R_{qu}^{(8)}$                                          | $(\bar{q}_p T^A u_r)(\bar{u}_s T^A q_t)$                                         | $R_{u^c d}$                  | $(\bar{u}_{\alpha p}^c d_{\beta r})(\bar{d}_{\beta s} u_{\alpha t}^c)$                                                                 |
| $R_{qd}^{(1)}$                                          | $(\bar{q}_p d_r)(\bar{d}_s q_t)$                                                 | $R'_{u^c d}$                 | $(\bar{u}_{\alpha p}^c d_{\beta r})(\bar{d}_{\alpha s} u_{\beta t}^c)$                                                                 |
| $R_{qd}^{(8)}$                                          | $(\bar{q}_p T^A d_r)(\bar{d}_s T^A q_t)$                                         |                              |                                                                                                                                        |
| $R_{\ell u q e}$                                        | $(\bar{\ell}_{ip} u_r) \epsilon^{ij} (\bar{q}_{js} e_t)$                         |                              |                                                                                                                                        |
| $(\bar{L}^c L)(\bar{L} L^c)$                            |                                                                                  | $(\bar{R}^c R)(\bar{L} L^c)$ |                                                                                                                                        |
| $R_{\ell^c \ell}$                                       | $(\bar{\ell}_{ip}^c \ell_{jr})(\bar{\ell}_{js} \ell_{it}^c)$                     | $R_{u^c d q q^c}$            | $(\bar{u}_{\alpha p}^c d_{\beta r}) \epsilon^{ij} (\bar{q}_{\beta is} q_{\alpha jt}^c)$                                                |
| $R_{q^c q}$                                             | $(\bar{q}_{\alpha ip}^c q_{\beta jr})(\bar{q}_{\beta js} q_{\alpha it}^c)$       | $R_{u^c e \ell q^c}$         | $(\bar{u}_p^c e_r) \epsilon^{ij} (\bar{\ell}_{is} q_{jt}^c)$                                                                           |
| $R'_{q^c q}$                                            | $(\bar{q}_{\alpha ip}^c q_{\beta jr})(\bar{q}_{\beta is} q_{\alpha jt}^c)$       | Baryon number violating      |                                                                                                                                        |
| $R_{q^c \ell}$                                          | $(\bar{q}_{ip}^c \ell_{jr})(\bar{\ell}_{js} \ell_{it}^c)$                        | $R_{q^c q q^c \ell}$         | $\epsilon_{\alpha\beta\gamma} \epsilon_{ij} \epsilon_{kl} (\bar{q}_{\alpha ip}^c q_{\beta jr})(\bar{q}_{\gamma ks} \ell_{lt}^c)$       |
| $R'_{q^c \ell}$                                         | $(\bar{q}_{ip}^c \ell_{jr})(\bar{\ell}_{is} q_{jt}^c)$                           | $R_{u^c u d^c e}$            | $\epsilon_{\alpha\beta\gamma} (\bar{u}_{\alpha p}^c u_{\beta r})(\bar{d}_{\gamma s}^c e_t)$                                            |
| Vector currents                                         |                                                                                  |                              |                                                                                                                                        |
| $(\bar{L}L)(\bar{L}L)$                                  |                                                                                  | $(\bar{L}^c R)(\bar{R}L^c)$  |                                                                                                                                        |
| $R_{\ell\ell}^{(3)}$                                    | $(\bar{\ell}_p \gamma_\mu \tau^I \ell_r)(\bar{\ell}_s \gamma^\mu \tau^I \ell_t)$ | $R_{\ell^c e}$               | $(\bar{\ell}_p^c \gamma_\mu e_r)(\bar{e}_s \gamma^\mu \ell_t^c)$                                                                       |
| $R_{qq}^{(1,8)}$                                        | $(\bar{q}_p \gamma_\mu T^A q_r)(\bar{q}_s \gamma^\mu T^A q_t)$                   | $R_{\ell^c u}$               | $(\bar{\ell}_p^c \gamma_\mu u_r)(\bar{u}_s \gamma^\mu \ell_t^c)$                                                                       |
| $R_{qq}^{(3,8)}$                                        | $(\bar{q}_p \gamma_\mu \tau^I T^A q_r)(\bar{q}_s \gamma^\mu \tau^I T^A q_t)$     | $R_{\ell^c d}$               | $(\bar{\ell}_p^c \gamma_\mu d_r)(\bar{d}_s \gamma^\mu \ell_t^c)$                                                                       |
| $R_{\ell q}^{(1)}$                                      | $(\bar{\ell}_p \gamma_\mu q_r)(\bar{q}_s \gamma^\mu \ell_t)$                     | $R_{q^c e d \ell^c}$         | $(\bar{q}_p^c \gamma^\mu e_r)(\bar{d}_s \gamma_\mu \ell_t^c)$                                                                          |
| $R_{\ell q}^{(3)}$                                      | $(\bar{\ell}_p \gamma_\mu \tau^I q_r)(\bar{q}_s \gamma^\mu \tau^I \ell_t)$       | $R_{q^c e}$                  | $(\bar{q}_p^c \gamma_\mu e_r)(\bar{e}_s \gamma^\mu q_t^c)$                                                                             |
| $(\bar{R}R)(\bar{R}R)$                                  |                                                                                  | $R_{q^c u}$                  | $(\bar{q}_{\alpha p}^c \gamma_\mu u_{\beta r})(\bar{u}_{\beta s} \gamma^\mu q_{\alpha t}^c)$                                           |
| $R_{uu}^{(8)}$                                          | $(\bar{u}_p \gamma_\mu T^A u_r)(\bar{u}_s \gamma^\mu T^A u_t)$                   | $R'_{q^c u}$                 | $(\bar{q}_{\alpha p}^c \gamma_\mu u_{\beta r})(\bar{u}_{\alpha s} \gamma^\mu q_{\beta t}^c)$                                           |
| $R_{dd}^{(8)}$                                          | $(\bar{d}_p \gamma_\mu T^A d_r)(\bar{d}_s \gamma^\mu T^A d_t)$                   | $R_{q^c d}$                  | $(\bar{q}_{\alpha p}^c \gamma_\mu d_{\beta r})(\bar{d}_{\beta s} \gamma^\mu q_{\alpha t}^c)$                                           |
| $R_{eu}$                                                | $(\bar{e}_p \gamma_\mu u_r)(\bar{u}_s \gamma^\mu e_t)$                           | $R'_{q^c d}$                 | $(\bar{q}_{\alpha p}^c \gamma_\mu d_{\beta r})(\bar{d}_{\alpha s} \gamma^\mu q_{\beta t}^c)$                                           |
| $R_{ed}$                                                | $(\bar{e}_p \gamma_\mu d_r)(\bar{d}_s \gamma^\mu e_t)$                           | Baryon number violating      |                                                                                                                                        |
| $R_{ud}^{(1)}$                                          | $(\bar{u}_p \gamma_\mu d_r)(\bar{d}_s \gamma^\mu u_t)$                           | $R_{d^c \ell q^c u}$         | $\epsilon_{\alpha\beta\gamma} \epsilon_{ij} (\bar{d}_{\alpha p}^c \gamma_\mu \ell_{ir})(\bar{q}_{\beta js}^c \gamma^\mu u_{\gamma t})$ |
| $R_{ud}^{(8)}$                                          | $(\bar{u}_p \gamma_\mu T^A d_r)(\bar{d}_s \gamma^\mu T^A u_t)$                   | $R_{u^c \ell q^c d}$         | $\epsilon_{\alpha\beta\gamma} \epsilon_{ij} (\bar{u}_{\alpha p}^c \gamma_\mu \ell_{ir})(\bar{q}_{\beta js}^c \gamma^\mu d_{\gamma t})$ |
| $(\bar{L}L)(\bar{R}R)$                                  |                                                                                  | $R_{q^c e u^c q}$            | $\epsilon_{\alpha\beta\gamma} \epsilon_{ij} (\bar{q}_{\alpha ip}^c \gamma_\mu e_r)(\bar{u}_{\beta s}^c \gamma^\mu q_{\gamma jt})$      |
| $R_{\ell q d e}$                                        | $(\bar{\ell}_p \gamma_\mu q_r)(\bar{d}_s \gamma^\mu e_t)$                        |                              |                                                                                                                                        |

Table 1: List of all redundant operators arising from tree-level matching.

## 2 List of Reduction Identities

We are now ready to list all reduction identities for the redundant operators in Table 1, including the full evanescent shifts. The results are tabulated below.

$$\begin{aligned}
R_{\ell e}^{prst} = & -\frac{1}{2}Q_{\ell e}^{ptsr} + \frac{1}{16\pi^2} \left[ \frac{1}{4}\overline{y_e^{uv}} y_e^{ts} Q_{\ell e}^{puvr} + \frac{1}{4}\overline{y_e^{pr}} y_e^{uv} Q_{\ell e}^{utsv} \right. \\
& + \frac{3}{8}g_Y \overline{y_e^{pr}} \overline{Q_{eB}^{ts}} + \frac{3}{8}g_Y y_e^{ts} Q_{eB}^{pr} + \frac{1}{2}\overline{y_e^{pr}} \overline{y_u^{uv}} \overline{Q_{\ell equ}^{(1)tsuv}} \\
& + \frac{1}{2}y_e^{ts} y_u^{uv} Q_{\ell equ}^{(1)pruv} + \overline{y_e^{pu}} \overline{y_e^{vr}} y_e^{vu} \overline{Q_{eH}^{ts}} + Q_{eH}^{pr} \left( \overline{y_e^{uv}} y_e^{tv} y_e^{us} \right. \\
& \left. - \frac{1}{2}\lambda y_e^{ts} \right) - \frac{1}{8}g_L \overline{y_e^{pr}} \overline{Q_{eW}^{ts}} - \frac{1}{8}g_L y_e^{ts} Q_{eW}^{pr} \\
& - \frac{1}{4}\overline{y_e^{ur}} y_e^{tv} Q_{\ell e}^{pusv} - \frac{1}{4}\overline{y_e^{pu}} y_e^{vs} Q_{\ell e}^{vtur} - \frac{1}{4}\overline{y_e^{ur}} y_e^{vs} Q_{\ell \ell}^{vupt} \\
& - \frac{1}{2}\lambda \overline{y_e^{pr}} \overline{Q_{eH}^{ts}} - \frac{1}{2}\mu^2 \overline{y_e^{pr}} \overline{Q_{ye}^{ts}} - \frac{1}{2}\overline{y_e^{pr}} y_d^{vu} \overline{Q_{\ell edq}^{tsuv}} \\
& \left. - \frac{1}{2}\overline{y_e^{pu}} y_e^{tv} Q_{ee}^{ursv} - \frac{1}{2}\overline{y_d^{uv}} y_e^{ts} Q_{\ell edq}^{prvu} - \frac{1}{2}\mu^2 y_e^{ts} Q_{ye}^{pr} \right]
\end{aligned} \tag{2.1}$$

$$\begin{aligned}
R_{\ell u}^{prst} = & -\frac{1}{2}Q_{\ell u}^{ptsr} + \frac{1}{16\pi^2} \left[ \frac{1}{16}\overline{y_e^{pu}} \overline{y_u^{vr}} \overline{Q_{\ell equ}^{(3)tuvs}} + \frac{1}{16}y_e^{tu} y_u^{vs} Q_{\ell equ}^{(3)puvr} \right. \\
& \left. - \frac{1}{4}\overline{y_u^{ur}} y_u^{vs} Q_{\ell q}^{(1)ptvu} - \frac{1}{2}\overline{y_e^{pu}} y_e^{tv} Q_{eu}^{uvsr} \right]
\end{aligned} \tag{2.2}$$

$$\begin{aligned}
R_{\ell d}^{prst} = & -\frac{1}{2}Q_{\ell d}^{ptsr} + \frac{1}{16\pi^2} \left[ \frac{1}{2}\overline{y_e^{pu}} y_d^{vs} \overline{Q_{\ell edq}^{turv}} + \frac{1}{2}\overline{y_d^{ur}} y_e^{tv} Q_{\ell edq}^{pvsu} \right. \\
& \left. - \frac{1}{4}\overline{y_d^{ur}} y_d^{vs} Q_{\ell q}^{(1)ptvu} - \frac{1}{2}\overline{y_e^{pu}} y_e^{tv} Q_{ed}^{uvsr} \right]
\end{aligned} \tag{2.3}$$

$$\begin{aligned}
R_{qe}^{prst} = & -\frac{1}{2}Q_{qe}^{ptsr} + \frac{1}{16\pi^2} \left[ \frac{1}{16}\overline{y_e^{ur}} \overline{y_u^{pv}} \overline{Q_{\ell equ}^{(3)ustv}} + \frac{1}{16}y_e^{us} y_u^{tv} Q_{\ell equ}^{(3)urpv} \right. \\
& + \frac{1}{2}\overline{y_e^{ur}} y_d^{tv} \overline{Q_{\ell edq}^{usvp}} + \frac{1}{2}\overline{y_d^{pu}} y_e^{vs} Q_{\ell edq}^{vrut} - \frac{1}{4}\overline{y_e^{ur}} y_e^{vs} Q_{\ell q}^{(1)vupt} \\
& \left. - \frac{1}{2}\overline{y_d^{pu}} y_d^{tv} Q_{ed}^{sruv} - \frac{1}{2}\overline{y_u^{pu}} y_u^{tv} Q_{eu}^{sruv} \right]
\end{aligned} \tag{2.4}$$

$$\begin{aligned}
R_{qu}^{(1)prst} = & -\frac{1}{6}Q_{qu}^{(1)ptsr} - Q_{qu}^{(8)ptsr} + \frac{1}{16\pi^2} \left[ \frac{1}{12}y_d^{tu} y_u^{vs} Q_{quqd}^{(1)vrpu} \right. \\
& + \frac{1}{4}\overline{y_u^{uv}} y_u^{ts} Q_{qu}^{(1)puvr} + \frac{1}{4}\overline{y_u^{pr}} y_u^{uv} Q_{qu}^{(1)utsv} + \frac{1}{2}y_d^{tu} y_u^{vs} Q_{quqd}^{(8)vrpu} \\
& + \overline{y_d^{pu}} \overline{y_u^{vr}} \left( \frac{1}{12}Q_{quqd}^{(1)vstu} + \frac{1}{2}Q_{quqd}^{(8)vstu} - \frac{1}{2}Q_{quqd}^{(1)tsvu} \right) \\
& + Q_{uH}^{pr} \left( 3\overline{y_u^{uv}} y_u^{tv} y_u^{us} - \frac{3}{2}\lambda y_u^{ts} \right) + \frac{3}{2}\overline{y_e^{uv}} \overline{y_u^{pr}} \overline{Q_{\ell equ}^{(1)uvts}} \\
& + \frac{3}{2}y_e^{uv} y_u^{ts} Q_{\ell equ}^{(1)uvpr} + \frac{3}{2}\overline{y_u^{uv}} y_u^{ts} Q_{qu}^{(8)puvr} + \frac{3}{2}\overline{y_u^{pr}} y_u^{uv} Q_{qu}^{(8)utsv} \\
& + 3\overline{y_u^{pu}} \overline{y_u^{vr}} y_u^{vu} \overline{Q_{uH}^{ts}} - \frac{1}{8}\overline{y_u^{ur}} y_u^{vs} Q_{qq}^{(1)vtpu} - \frac{1}{8}\overline{y_u^{ur}} y_u^{vs} Q_{qq}^{(3)vtpu}
\end{aligned} \tag{2.5}$$

$$\begin{aligned}
& -\frac{1}{6}\overline{y_d^{pu}} y_d^{tv} Q_{ud}^{(1)sruv} - \frac{1}{4}\overline{y_u^{ur}} y_u^{tv} Q_{qu}^{(1)pusv} - \frac{1}{4}\overline{y_u^{pu}} y_u^{vs} Q_{qu}^{(1)vtur} \\
& -\frac{3}{8}g_L\overline{y_u^{pr}} \overline{Q_{uW}^{ts}} - \frac{3}{8}g_L y_u^{ts} Q_{uW}^{pr} - \frac{1}{2}y_d^{tu} y_u^{vs} Q_{quqd}^{(1)prvu} \\
& -\frac{1}{2}\overline{y_u^{pu}} y_u^{tv} Q_{uu}^{ursv} - \frac{5}{8}g_Y\overline{y_u^{pr}} \overline{Q_{uB}^{ts}} - \frac{5}{8}g_Y y_u^{ts} Q_{uB}^{pr} \\
& -\overline{y_d^{pu}} y_d^{tv} Q_{ud}^{(8)sruv} - \frac{3}{2}\overline{y_d^{uv}} \overline{y_u^{pr}} \overline{Q_{quqd}^{(1)tsuv}} - \frac{3}{2}\lambda\overline{y_u^{pr}} \overline{Q_{uH}^{ts}} \\
& -\frac{3}{2}\mu^2\overline{y_u^{pr}} \overline{Q_{yu}^{ts}} - \frac{3}{2}y_d^{uv} y_u^{ts} Q_{quqd}^{(1)pruv} - \frac{3}{2}\mu^2 y_u^{ts} Q_{yu}^{pr} \Big]
\end{aligned}$$

$$\begin{aligned}
R_{qu}^{(8)prst} = & \frac{1}{6}Q_{qu}^{(8)ptsr} - \frac{2}{9}Q_{qu}^{(1)ptsr} + \frac{1}{16\pi^2} \Big[ \frac{1}{48}\overline{y_u^{ur}} y_u^{vs} Q_{qq}^{(1)puvt} \\
& + \frac{1}{48}\overline{y_u^{ur}} y_u^{vs} Q_{qq}^{(3)puvt} + \frac{1}{12}\overline{y_u^{pu}} y_u^{tv} Q_{uu}^{ursv} + \frac{1}{9}y_d^{tu} y_u^{vs} Q_{quqd}^{(1)vrpu} \\
& + \frac{1}{6}\overline{y_d^{pu}} y_d^{tv} Q_{ud}^{(8)sruv} + \overline{y_d^{pu}} \overline{y_u^{vr}} \left( \frac{1}{9}\overline{Q_{quqd}^{(1)vstu}} - \frac{1}{12}\overline{Q_{quqd}^{(8)vstu}} \right. \\
& \left. - \frac{1}{2}\overline{Q_{quqd}^{(8)tsvu}} \right) - \frac{1}{12}y_d^{tu} y_u^{vs} Q_{quqd}^{(8)vrpu} - \frac{1}{8}\overline{y_u^{ur}} y_u^{vs} Q_{qq}^{(1)vuqt} \\
& - \frac{2}{9}\overline{y_d^{pu}} y_d^{tv} Q_{ud}^{(1)sruv} - \frac{1}{4}g_s\overline{y_u^{pr}} \overline{Q_{uG}^{ts}} - \frac{1}{4}\overline{y_u^{ur}} y_u^{tv} Q_{qu}^{(8)pusv} \\
& - \frac{1}{4}\overline{y_u^{pu}} y_u^{vs} Q_{qu}^{(8)vtur} - \frac{1}{4}g_s y_u^{ts} Q_{uG}^{pr} - \frac{1}{4}\overline{y_u^{pu}} y_u^{tv} Q_{uu}^{uvsr} \\
& \left. - \frac{1}{2}y_d^{tu} y_u^{vs} Q_{quqd}^{(8)prvu} \right]
\end{aligned} \tag{2.6}$$

$$\begin{aligned}
R_{qd}^{(1)prst} = & -\frac{1}{6}Q_{qd}^{(1)ptsr} - Q_{qd}^{(8)ptsr} + \frac{1}{16\pi^2} \Big[ \frac{1}{12}y_d^{us} y_u^{tv} Q_{quqd}^{(1)pvur} \\
& + \frac{1}{8}g_Y\overline{y_d^{pr}} \overline{Q_{dB}^{ts}} + \frac{1}{8}g_Y y_d^{ts} Q_{dB}^{pr} + \frac{1}{4}\overline{y_d^{uv}} y_d^{ts} Q_{qd}^{(1)puvr} \\
& + \frac{1}{4}\overline{y_d^{pr}} y_d^{uv} Q_{qd}^{(1)utsv} + \frac{1}{2}y_d^{us} y_u^{tv} Q_{quqd}^{(8)pvur} + \overline{y_d^{ur}} \overline{y_u^{pv}} \left( \frac{1}{12}\overline{Q_{quqd}^{(1)tvus}} \right. \\
& \left. + \frac{1}{2}\overline{Q_{quqd}^{(8)tvus}} - \frac{1}{2}\overline{Q_{quqd}^{(1)uvtst}} \right) + Q_{dH}^{pr} \left( 3\overline{y_d^{uv}} y_d^{tv} y_d^{us} \right. \\
& \left. - \frac{3}{2}\lambda y_d^{ts} \right) + Q_{quqd}^{(1)uvpr} \left( -\frac{1}{2}y_d^{us} y_u^{tv} \right. \\
& \left. - \frac{3}{2}y_d^{ts} y_u^{uv} \right) + \frac{3}{2}\overline{y_d^{uv}} y_d^{ts} Q_{qd}^{(8)puvr} + \frac{3}{2}\overline{y_d^{pr}} y_d^{uv} Q_{qd}^{(8)utsv} \\
& + 3\overline{y_d^{pu}} \overline{y_d^{vr}} y_d^{vu} \overline{Q_{dH}^{ts}} - \frac{1}{8}\overline{y_d^{ur}} y_d^{vs} Q_{qq}^{(1)vtpu} - \frac{1}{8}\overline{y_d^{ur}} y_d^{vs} Q_{qq}^{(3)vtpu} \\
& - \frac{1}{6}\overline{y_u^{pu}} y_u^{tv} Q_{ud}^{(1)uvsr} - \frac{1}{4}\overline{y_d^{ur}} y_d^{tv} Q_{qd}^{(1)pusv} - \frac{1}{4}\overline{y_d^{pu}} y_d^{vs} Q_{qd}^{(1)vtur} \\
& - \frac{3}{8}g_L\overline{y_d^{pr}} \overline{Q_{dW}^{ts}} - \frac{3}{8}g_L y_d^{ts} Q_{dW}^{pr} - \frac{1}{2}\overline{y_d^{pu}} y_d^{tv} Q_{dd}^{ursv} \\
& - \overline{y_u^{pu}} y_u^{tv} Q_{ud}^{(8)uvsr} - \frac{3}{2}\overline{y_d^{pr}} \overline{y_u^{uv}} \overline{Q_{quqd}^{(1)uvtst}} - \frac{3}{2}\lambda\overline{y_d^{pr}} \overline{Q_{dH}^{ts}} \\
& - \frac{3}{2}\mu^2\overline{y_d^{pr}} \overline{Q_{yd}^{ts}} - \frac{3}{2}y_e^{uv} y_d^{ts} Q_{ledq}^{uvrp} - \frac{3}{2}\overline{y_d^{pr}} y_e^{uv} Q_{ledq}^{uvst} \\
& \left. - \frac{3}{2}\mu^2 y_d^{ts} Q_{yd}^{pr} \right]
\end{aligned} \tag{2.7}$$

$$\begin{aligned}
R_{qd}^{(8)prst} = & \frac{1}{6}Q_{qd}^{(8)ptsr} - \frac{2}{9}Q_{qd}^{(1)ptsr} + \frac{1}{16\pi^2} \left[ \frac{1}{48}\overline{y_d^{ur}} y_d^{vs} Q_{qq}^{(1)puvt} \right. \\
& + \frac{1}{48}\overline{y_d^{ur}} y_d^{vs} Q_{qq}^{(3)puvt} + \frac{1}{12}\overline{y_d^{pu}} y_d^{tv} Q_{dd}^{ursv} + \frac{1}{9}y_d^{us} y_u^{tv} Q_{quqd}^{(1)pvur} \\
& + \frac{1}{6}\overline{y_u^{pu}} y_u^{tv} Q_{ud}^{(8)uvsr} + \overline{y_d^{ur}} \overline{y_u^{pv}} \left( \frac{1}{9}\overline{Q_{quqd}^{(1)tvus}} - \frac{1}{12}\overline{Q_{quqd}^{(8)tvus}} \right. \\
& \left. \left. - \frac{1}{2}\overline{Q_{quqd}^{(8)uvt s}} \right) - \frac{1}{12}y_d^{us} y_u^{tv} Q_{quqd}^{(8)pvur} - \frac{1}{8}\overline{y_d^{ur}} y_d^{vs} Q_{qq}^{(1)vu pt} \right. \\
& - \frac{2}{9}\overline{y_u^{pu}} y_u^{tv} Q_{ud}^{(1)uvsr} - \frac{1}{4}g_s \overline{y_d^{pr}} \overline{Q_{dG}^{ts}} - \frac{1}{4}\overline{y_d^{pu}} y_d^{tv} Q_{dd}^{uvsr} \\
& - \frac{1}{4}g_s y_d^{ts} Q_{dG}^{pr} - \frac{1}{4}\overline{y_d^{ur}} y_d^{tv} Q_{qd}^{(8)pusv} - \frac{1}{4}\overline{y_d^{pu}} y_d^{vs} Q_{qd}^{(8)vtur} \\
& \left. \left. - \frac{1}{2}y_d^{us} y_u^{tv} Q_{quqd}^{(8)uvpr} \right] \right.
\end{aligned} \tag{2.8}$$

$$\begin{aligned}
R_{luqe}^{prst} = & -\frac{1}{8}Q_{lequ}^{(3)ptsr} - \frac{1}{2}Q_{lequ}^{(1)ptsr} + \frac{1}{16\pi^2} \left[ \frac{1}{32}\overline{y_e^{ut}} \overline{y_u^{vr}} Q_{\ell q}^{(3)pusv} \right. \\
& + \frac{1}{4}\overline{y_d^{su}} \overline{y_u^{vr}} Q_{\ell edq}^{ptuv} + \frac{3}{8}g_L \overline{y_u^{sr}} Q_{eW}^{pt} (\xi_{rp} - 1) \\
& + Q_{lequ}^{(1)ptsr} \left( \frac{85}{72}g_Y^2 + \frac{15}{8}g_L^2 - \frac{7}{3}g_s^2 \right) \\
& + Q_{lequ}^{(3)ptsr} \left( \frac{1}{12}g_s^2 - \frac{25}{288}g_Y^2 - \frac{3}{32}g_L^2 \right) \\
& - \frac{1}{32}\overline{y_e^{ut}} \overline{y_u^{vr}} Q_{\ell q}^{(1)pusv} - \frac{1}{8}\overline{y_e^{pu}} \overline{y_u^{sv}} Q_{eu}^{utvr} - \frac{3}{16}\overline{y_e^{ut}} \overline{y_u^{sv}} Q_{\ell u}^{puvr} \\
& \left. - \frac{3}{16}\overline{y_e^{pu}} \overline{y_u^{vr}} Q_{qe}^{svut} - \frac{5}{8}g_Y \overline{y_u^{sr}} Q_{eB}^{pt} (\xi_{rp} - 1) \right]
\end{aligned} \tag{2.9}$$

$$\begin{aligned}
R_{\ell c \ell}^{prst} = & \frac{1}{2}Q_{\ell \ell}^{srtp} + \frac{1}{16\pi^2} \left[ \frac{1}{18}g_Y^2 \delta^{rt} Q_{\ell q}^{(1)s puu} + \frac{2}{9}g_Y^2 \delta^{rt} Q_{\ell u}^{s puu} \right. \\
& + Q_{H\ell}^{(1)sp} \left( \frac{1}{6}g_Y^2 \delta^{rt} + \frac{1}{2}\overline{y_e^{tu}} y_e^{ru} \right) + Q_{H\ell}^{(3)sp} \left( \frac{1}{2}\overline{y_e^{tu}} y_e^{ru} \right. \\
& \left. - \frac{1}{6}g_L^2 \delta^{rt} \right) + \overline{y_e^{tu}} y_e^{rv} Q_{\ell e}^{spuv} + \overline{y_e^{su}} y_e^{rv} Q_{\ell e}^{tpuv} \\
& + Q_{\ell \ell}^{srtp} \left( \frac{3}{4}g_Y^2 - \frac{3}{4}g_L^2 \right) + Q_{\ell \ell}^{uus p} \left( \frac{1}{6}g_L^2 \delta^{rt} \right. \\
& \left. - \frac{1}{6}g_Y^2 \delta^{rt} \right) + \frac{3}{2}g_L^2 Q_{\ell \ell}^{trsp} - \frac{1}{9}g_Y^2 \delta^{rt} Q_{\ell d}^{s puu} \\
& \left. - \frac{1}{6}g_L^2 \delta^{rt} Q_{\ell q}^{(3)s puu} - \frac{1}{3}g_Y^2 \delta^{rt} Q_{\ell e}^{s puu} - \frac{1}{3}g_L^2 \delta^{rt} Q_{\ell \ell}^{upsu} \right]
\end{aligned} \tag{2.10}$$

$$\begin{aligned}
R_{q^c q}^{prst} = & \frac{1}{2}Q_{qq}^{(1)srtp} + \frac{1}{16\pi^2} \left[ \frac{1}{27}g_Y^2 \delta^{rt} Q_{qd}^{(1)s puu} + \frac{1}{18}g_Y^2 \delta^{rt} Q_{\ell q}^{(1)uus p} \right. \\
& + \frac{1}{9}g_Y^2 \delta^{rt} Q_{qe}^{s puu} + \frac{1}{3}\overline{y_d^{tu}} y_d^{rv} Q_{qd}^{(1)s puv} + \frac{1}{3}\overline{y_u^{tu}} y_u^{rv} Q_{qu}^{(1)s puv} \\
& + \frac{3}{4}g_s^2 Q_{qq}^{(1)trsp} + \frac{3}{4}g_L^2 Q_{qq}^{(3)tps r} + \frac{3}{4}g_s^2 Q_{qq}^{(3)trsp} \\
& \left. + \overline{y_d^{tu}} \overline{y_u^{sv}} \left( \frac{1}{3}\overline{Q_{quqd}^{(1)pvru}} + 2\overline{Q_{quqd}^{(8)pvru}} \right) + Q_{Hq}^{(1)sp} \left( \frac{1}{2}\overline{y_d^{tu}} y_d^{ru} \right. \right.
\end{aligned} \tag{2.11}$$

$$\begin{aligned}
& -\frac{1}{18}g_Y^2\delta^{rt} - \frac{1}{2}\overline{y_u^{tu}} y_u^{ru} \Big) + Q_{Hq}^{(3)sp} \Big( \frac{1}{2}\overline{y_d^{tu}} y_d^{ru} \\
& + \frac{1}{2}\overline{y_u^{tu}} y_u^{ru} - \frac{1}{6}g_L^2\delta^{rt} \Big) + \overline{y_d^{su}} y_d^{rv} Q_{qd}^{(1)tpuv} \\
& + Q_{qq}^{(1)srt p} \Big( \frac{1}{12}g_Y^2 - \frac{1}{2}g_s^2 \Big) + Q_{qq}^{(1)uusp} \Big( \frac{1}{9}g_s^2\delta^{rt} \\
& - \frac{1}{54}g_Y^2\delta^{rt} \Big) + \overline{y_u^{su}} y_u^{rv} Q_{qu}^{(1)tpuv} + Q_{quqd}^{(1)svtu} \Big( \frac{1}{3}y_d^{ru} y_u^{pv} \\
& - \frac{1}{2}y_d^{pu} y_u^{rv} \Big) + 2\overline{y_d^{tu}} y_d^{rv} Q_{qd}^{(8)spuv} + 2\overline{y_u^{tu}} y_u^{rv} Q_{qu}^{(8)spuv} \\
& + 2y_d^{ru} y_u^{pv} Q_{quqd}^{(8)svtu} - \frac{2}{27}g_Y^2\delta^{rt} Q_{qu}^{(1)spuu} - \frac{1}{6}g_L^2\delta^{rt} Q_{\ell q}^{(3)uusp} \\
& - \frac{1}{6}g_s^2\delta^{rt} Q_{qq}^{(1)upsu} - \frac{1}{6}g_s^2\delta^{rt} Q_{qq}^{(3)upsu} - \frac{1}{6}g_L^2\delta^{rt} Q_{qq}^{(3)uusp} \\
& - \frac{1}{2}\overline{y_d^{su}} \overline{y_u^{tv}} \overline{Q_{quqd}^{(1)pvr u}} - \frac{2}{3}g_s^2\delta^{rt} Q_{qd}^{(8)spuu} - \frac{2}{3}g_s^2\delta^{rt} Q_{qu}^{(8)spuu} \Big]
\end{aligned}$$

$$R_{q^c q}^{prst} = \frac{1}{4}Q_{qq}^{(1)srt p} + \frac{1}{4}Q_{qq}^{(3)srt p} + \frac{1}{16\pi^2} \Big[ \frac{2}{27}g_Y^2\delta^{rt} Q_{qd}^{(1)spuu} \quad (2.12)$$

$$\begin{aligned}
& + \frac{1}{9}g_Y^2\delta^{rt} Q_{\ell q}^{(1)uusp} + \frac{2}{9}g_Y^2\delta^{rt} Q_{qe}^{spuu} + \frac{1}{2}\overline{y_d^{su}} \overline{y_u^{tv}} \overline{Q_{quqd}^{(1)pvr u}} \\
& + \frac{1}{2}\overline{y_d^{su}} y_d^{rv} Q_{qd}^{(1)tpuv} + \frac{1}{2}\overline{y_u^{su}} y_u^{rv} Q_{qu}^{(1)tpuv} + \frac{2}{3}\overline{y_d^{tu}} y_d^{rv} Q_{qd}^{(1)spuv} \\
& + \frac{2}{3}\overline{y_u^{tu}} y_u^{rv} Q_{qu}^{(1)spuv} + \overline{y_d^{tu}} \overline{y_u^{sv}} \Big( -\frac{1}{3}Q_{quqd}^{(1)pvr u} \\
& - 2Q_{quqd}^{(8)pvr u} \Big) + Q_{Hq}^{(1)sp} \Big( \overline{y_d^{tu}} y_d^{ru} - \frac{1}{9}g_Y^2\delta^{rt} \\
& - \overline{y_u^{tu}} y_u^{ru} \Big) + Q_{qq}^{(1)srt p} \Big( \frac{1}{24}g_Y^2 + \frac{9}{8}g_L^2 \\
& - \frac{1}{4}g_s^2 \Big) + Q_{qq}^{(1)uusp} \Big( \frac{2}{9}g_s^2\delta^{rt} - \frac{1}{27}g_Y^2\delta^{rt} \Big) \\
& + Q_{qq}^{(3)srt p} \Big( \frac{1}{24}g_Y^2 - \frac{1}{4}g_s^2 - \frac{3}{8}g_L^2 \Big) \\
& + Q_{quqd}^{(1)svtu} \Big( \frac{1}{2}y_d^{pu} y_u^{rv} - \frac{1}{3}y_d^{ru} y_u^{pv} \Big) + \frac{3}{2}g_s^2 Q_{qq}^{(1)spt r} \\
& + 4\overline{y_d^{tu}} y_d^{rv} Q_{qd}^{(8)spuv} + 4\overline{y_u^{tu}} y_u^{rv} Q_{qu}^{(8)spuv} - \frac{4}{27}g_Y^2\delta^{rt} Q_{qu}^{(1)spuu} \\
& - \frac{1}{3}g_s^2\delta^{rt} Q_{qq}^{(1)upsu} - \frac{1}{3}g_s^2\delta^{rt} Q_{qq}^{(3)upsu} - \frac{4}{3}g_s^2\delta^{rt} Q_{qd}^{(8)spuu} \\
& - \frac{4}{3}g_s^2\delta^{rt} Q_{qu}^{(8)spuu} - 2y_d^{ru} y_u^{pv} Q_{quqd}^{(8)svtu} \Big]
\end{aligned}$$

$$R_{q^c \ell}^{prst} = \frac{1}{2}Q_{\ell q}^{(1)srt p} + \frac{1}{16\pi^2} \Big[ \frac{1}{2}\overline{y_d^{tu}} y_d^{pv} Q_{\ell d}^{sruv} + \frac{1}{2}\overline{y_u^{tu}} y_u^{pv} Q_{\ell u}^{sruv} \quad (2.13)$$

$$\begin{aligned}
& + \frac{1}{2}\overline{y_e^{su}} y_e^{rv} Q_{qe}^{tpuv} + \frac{3}{4}g_L^2 Q_{\ell q}^{(3)srt p} + Q_{\ell q}^{(1)srt p} \Big( \frac{1}{6}g_Y^2 \\
& + 2g_s^2 + \frac{9}{4}g_L^2 \Big) - \frac{1}{16}\overline{y_e^{su}} \overline{y_u^{tv}} \overline{Q_{\ell equ}^{(3)rupv}} \\
& - \frac{1}{16}y_e^{ru} y_u^{pv} Q_{\ell equ}^{(3)sutv} - \overline{y_e^{su}} y_d^{pv} \overline{Q_{\ell edq}^{ruvt}} - \overline{y_d^{tu}} y_e^{rv} Q_{\ell edq}^{svup} \Big]
\end{aligned}$$

$$\begin{aligned}
R_{q^c \ell}^{prst} = & \frac{1}{4} Q_{\ell q}^{(1)srt p} + \frac{1}{4} Q_{\ell q}^{(3)srt p} + \frac{1}{16\pi^2} \left[ \frac{1}{16} \overline{y_e^{su}} \overline{y_u^{tv}} \overline{Q_{\ell equ}^{(3)rupv}} \right. \\
& + \frac{1}{16} y_e^{ru} y_u^{pv} Q_{\ell equ}^{(3)sutv} + \frac{1}{4} \overline{y_d^{tu}} y_d^{pv} Q_{\ell d}^{sruv} + \frac{1}{4} \overline{y_u^{tu}} y_u^{pv} Q_{\ell u}^{sruv} \\
& + \frac{1}{4} \overline{y_e^{su}} y_e^{rv} Q_{qe}^{tpuv} + Q_{\ell q}^{(1)srt p} \left( \frac{1}{12} g_Y^2 + g_s^2 \right. \\
& + \frac{9}{4} g_L^2 \left. \right) + Q_{\ell q}^{(3)srt p} \left( \frac{1}{12} g_Y^2 + g_s^2 \right. \\
& \left. \left. - \frac{3}{4} g_L^2 \right) - 2 \overline{y_e^{su}} y_d^{pv} \overline{Q_{\ell edq}^{ruvt}} - 2 \overline{y_d^{tu}} y_e^{rv} Q_{\ell edq}^{svup} \right]
\end{aligned} \tag{2.14}$$

$$\begin{aligned}
R_{e^c e}^{prst} = & \frac{1}{2} Q_{ee}^{srt p} + \frac{1}{16\pi^2} \left[ \frac{1}{9} g_Y^2 \delta^{rt} Q_{qe}^{uusp} + \frac{4}{9} g_Y^2 \delta^{rt} Q_{eu}^{spuu} \right. \\
& + Q_{He}^{sp} \left( \frac{1}{3} g_Y^2 \delta^{rt} - \overline{y_e^{ur}} y_e^{ut} \right) + \frac{3}{2} \overline{y_e^{up}} y_e^{vt} Q_{\ell e}^{vusr} \\
& + 3 g_Y^2 Q_{ee}^{spt r} - \frac{2}{9} g_Y^2 \delta^{rt} Q_{ed}^{spuu} - \frac{1}{3} g_Y^2 \delta^{rt} Q_{\ell e}^{uusp} \\
& \left. - \frac{2}{3} g_Y^2 \delta^{rt} Q_{ee}^{spuu} \right]
\end{aligned} \tag{2.15}$$

$$\begin{aligned}
R_{u^c u}^{prst} = & \frac{1}{2} Q_{uu}^{srt p} + \frac{1}{16\pi^2} \left[ \frac{4}{27} g_Y^2 \delta^{ps} Q_{ud}^{(1)truu} + \frac{2}{9} g_Y^2 \delta^{rt} Q_{\ell u}^{uusp} \right. \\
& + \frac{1}{3} \overline{y_u^{ur}} y_u^{vt} Q_{qu}^{(1)vusp} + \frac{4}{9} g_Y^2 \delta^{rt} Q_{eu}^{uusp} + \frac{1}{2} \overline{y_u^{up}} y_u^{vt} Q_{qu}^{(1)vusr} \\
& + Q_{Hu}^{sp} \left( \overline{y_u^{ur}} y_u^{ut} - \frac{2}{9} g_Y^2 \delta^{rt} \right) + Q_{uu}^{srt p} \left( \frac{4}{3} g_Y^2 \right. \\
& - \frac{1}{2} g_s^2 \left. \right) + Q_{uu}^{uutr} \left( \frac{1}{9} g_s^2 \delta^{ps} - \frac{8}{27} g_Y^2 \delta^{ps} \right) \\
& + \frac{3}{2} g_s^2 Q_{uu}^{spt r} + 2 \overline{y_u^{ur}} y_u^{vt} Q_{qu}^{(8)vusp} - \frac{2}{27} g_Y^2 \delta^{rt} Q_{qu}^{(1)uusp} \\
& \left. - \frac{1}{3} g_s^2 \delta^{ps} Q_{uu}^{urtu} - \frac{2}{3} g_s^2 \delta^{rt} Q_{qu}^{(8)uusp} - \frac{2}{3} g_s^2 \delta^{ps} Q_{ud}^{(8)truu} \right]
\end{aligned} \tag{2.16}$$

$$\begin{aligned}
R_{d^c d}^{prst} = & \frac{1}{2} Q_{dd}^{srt p} + \frac{1}{16\pi^2} \left[ \frac{1}{27} g_Y^2 \delta^{rt} Q_{qd}^{(1)uusp} + \frac{4}{27} g_Y^2 \delta^{ps} Q_{ud}^{(1)uutr} \right. \\
& + \frac{1}{3} \overline{y_d^{ur}} y_d^{vt} Q_{qd}^{(1)vusp} + \frac{1}{2} \overline{y_d^{up}} y_d^{vt} Q_{qd}^{(1)vusr} + Q_{dd}^{srt p} \left( \frac{1}{3} g_Y^2 \right. \\
& - \frac{1}{2} g_s^2 \left. \right) + Q_{dd}^{uusp} \left( \frac{1}{9} g_s^2 \delta^{rt} - \frac{2}{27} g_Y^2 \delta^{rt} \right) \\
& + Q_{Hd}^{sp} \left( \frac{1}{9} g_Y^2 \delta^{rt} - \overline{y_d^{ur}} y_d^{ut} \right) + \frac{3}{2} g_s^2 Q_{dd}^{spt r} \\
& + 2 \overline{y_d^{ur}} y_d^{vt} Q_{qd}^{(8)vusp} - \frac{1}{9} g_Y^2 \delta^{rt} Q_{\ell d}^{uusp} - \frac{2}{9} g_Y^2 \delta^{rt} Q_{ed}^{uusp} \\
& \left. - \frac{1}{3} g_s^2 \delta^{rt} Q_{dd}^{upsu} - \frac{2}{3} g_s^2 \delta^{rt} Q_{qd}^{(8)uusp} - \frac{2}{3} g_s^2 \delta^{ps} Q_{ud}^{(8)uutr} \right]
\end{aligned} \tag{2.17}$$

$$\begin{aligned}
R_{e^c u}^{prst} = & \frac{1}{2} Q_{eu}^{tpsr} + \frac{1}{16\pi^2} \left[ \frac{1}{4} \overline{y_e^{up}} y_e^{vt} Q_{\ell u}^{vusr} + \frac{1}{4} \overline{y_u^{ur}} y_u^{vs} Q_{qe}^{vutp} \right. \\
& + Q_{eu}^{tpsr} \left( \frac{1}{6} g_Y^2 + 2 g_s^2 \right) - \frac{1}{16} \overline{y_e^{up}} \overline{y_u^{vr}} \overline{Q_{\ell equ}^{(3)utvs}}
\end{aligned} \tag{2.18}$$



$$\begin{aligned}
& -\frac{1}{16}y_e^{ut}y_u^{vs}Q_{\ell equ}^{(3)upvr} \Big] \\
R_{ecd}^{prst} = & \frac{1}{2}Q_{ed}^{tpsr} + \frac{1}{16\pi^2} \left[ \frac{1}{4}\overline{y_e^{up}} y_e^{vt}Q_{\ell d}^{vusr} + \frac{1}{4}\overline{y_d^{ur}} y_d^{vs}Q_{qe}^{vutp} \right. \\
& + Q_{ed}^{tpsr} \left( 2g_s^2 + \frac{8}{3}g_Y^2 \right) - \overline{y_e^{up}} y_d^{vs}Q_{\ell edq}^{utrv} \\
& \left. - \overline{y_d^{ur}} y_e^{vt}Q_{\ell edq}^{vpsu} \right]
\end{aligned} \tag{2.19}$$

$$\begin{aligned}
R_{ucd}^{prst} = & \frac{1}{2}Q_{ud}^{(1)tpsr} + \frac{1}{16\pi^2} \left[ \frac{1}{6}y_d^{us}y_u^{vt}Q_{quqd}^{(1)upvr} + \frac{1}{4}\overline{y_u^{up}} y_u^{vt}Q_{qd}^{(1)vusr} \right. \\
& + \frac{1}{4}\overline{y_d^{ur}} y_d^{vs}Q_{qu}^{(1)vutp} + \overline{y_d^{ur}} \overline{y_u^{vp}} \left( \frac{1}{6}\overline{Q_{quqd}^{(1)utvs}} + \overline{Q_{quqd}^{(8)utvs}} \right. \\
& \left. \left. - \frac{1}{4}\overline{Q_{quqd}^{(1)vtus}} \right) + y_d^{us}y_u^{vt}Q_{quqd}^{(8)upvr} + Q_{ud}^{(1)tpsr} \left( \frac{1}{6}g_Y^2 \right. \right. \\
& \left. \left. + 4g_s^2 \right) + 3g_s^2Q_{ud}^{(8)tpsr} - \frac{1}{4}y_d^{us}y_u^{vt}Q_{quqd}^{(1)vpur} \right. \\
& \left. - \overline{y_d^{ur}} y_u^{vt}Q_{Hud}^{ps} - \overline{y_u^{up}} y_d^{us}Q_{Hud}^{tr} \right]
\end{aligned} \tag{2.20}$$

$$\begin{aligned}
R_{ucd}^{prst} = & \frac{1}{6}Q_{ud}^{(1)tpsr} + Q_{ud}^{(8)tpsr} + \frac{1}{16\pi^2} \left[ \frac{1}{12}\overline{y_u^{up}} y_u^{vt}Q_{qd}^{(1)vusr} \right. \\
& + \frac{1}{12}\overline{y_d^{ur}} y_d^{vs}Q_{qu}^{(1)vutp} + \frac{1}{2}\overline{y_u^{up}} y_u^{vt}Q_{qd}^{(8)vusr} + \frac{1}{2}\overline{y_d^{ur}} y_d^{vs}Q_{qu}^{(8)vutp} \\
& + \frac{1}{2}y_d^{us}y_u^{vt}Q_{quqd}^{(1)upvr} + \overline{y_d^{ur}} \overline{y_u^{vp}} \left( \frac{1}{2}\overline{Q_{quqd}^{(1)utvs}} - \frac{1}{12}\overline{Q_{quqd}^{(1)vtus}} \right. \\
& \left. \left. - \frac{1}{2}\overline{Q_{quqd}^{(8)vtus}} \right) + Q_{ud}^{(1)tpsr} \left( \frac{1}{18}g_Y^2 + \frac{8}{3}g_s^2 \right) \right. \\
& + Q_{ud}^{(8)tpsr} \left( \frac{1}{3}g_Y^2 - 2g_s^2 \right) - \frac{1}{12}y_d^{us}y_u^{vt}Q_{quqd}^{(1)vpur} \\
& \left. - \frac{1}{2}y_d^{us}y_u^{vt}Q_{quqd}^{(8)vpur} - 3\overline{y_d^{ur}} y_u^{vt}Q_{Hud}^{ps} - 3\overline{y_u^{up}} y_d^{us}Q_{Hud}^{tr} \right]
\end{aligned} \tag{2.21}$$

$$\begin{aligned}
R_{ucdq}^{prst} = & Q_{quqd}^{(1)tpsr} - \frac{1}{3}Q_{quqd}^{(1)sptr} - 2Q_{quqd}^{(8)sptr} \\
& + \frac{1}{16\pi^2} \left[ \frac{1}{8}\overline{y_d^{ur}} \overline{y_u^{vp}} Q_{qq}^{(3)sutv} + \frac{1}{4}\overline{y_d^{su}} \overline{y_u^{vp}} Q_{qd}^{(1)tvur} + \frac{1}{4}\overline{y_d^{ur}} \overline{y_u^{tv}} Q_{qu}^{(1)suvp} \right. \\
& + Q_{quqd}^{(1)sptr} \left( \frac{35}{216}g_Y^2 + \frac{7}{8}g_L^2 - \frac{56}{9}g_s^2 \right) \\
& + Q_{quqd}^{(1)tpsr} \left( \frac{28}{3}g_s^2 - \frac{35}{72}g_Y^2 - \frac{21}{8}g_L^2 \right) \\
& + Q_{quqd}^{(8)sptr} \left( \frac{35}{36}g_Y^2 + \frac{14}{3}g_s^2 + \frac{21}{4}g_L^2 \right) \\
& + Q_{ud}^{(1)vpur} \left( \frac{1}{6}\overline{y_d^{tu}} \overline{y_u^{sv}} - \frac{1}{2}\overline{y_d^{su}} \overline{y_u^{tv}} \right) + \overline{y_d^{tu}} \overline{y_u^{sv}} Q_{ud}^{(8)vpur} \\
& + 7g_s^2Q_{quqd}^{(8)tpsr} - \frac{1}{12}\overline{y_d^{tu}} \overline{y_u^{vp}} Q_{qd}^{(1)svur} - \frac{1}{12}\overline{y_d^{ur}} \overline{y_u^{sv}} Q_{qu}^{(1)tuvp} \\
& \left. - \frac{1}{8}\overline{y_d^{ur}} \overline{y_u^{vp}} Q_{qq}^{(1)tvsu} - \frac{1}{2}\overline{y_d^{tu}} \overline{y_u^{vp}} Q_{qd}^{(8)svur} - \frac{1}{2}\overline{y_d^{ur}} \overline{y_u^{sv}} Q_{qu}^{(8)tuvp} \right]
\end{aligned} \tag{2.22}$$

$$\begin{aligned}
R_{u^c e l q^c}^{prst} = & \frac{1}{8} Q_{lequ}^{(3)srt p} - \frac{1}{2} Q_{lequ}^{(1)srt p} + \frac{1}{16\pi^2} \left[ \frac{3}{32} \overline{y_e^{ur}} \overline{y_u^{vp}} Q_{lq}^{(3)sutv} \right. \\
& + \frac{1}{4} \overline{y_d^{tu}} \overline{y_u^{vp}} Q_{ledq}^{sruv} + \frac{7}{16} \overline{y_e^{ur}} \overline{y_u^{tv}} Q_{lu}^{suvp} + \frac{7}{16} \overline{y_e^{su}} \overline{y_u^{vp}} Q_{qe}^{tvur} \\
& + \frac{5}{8} g_Y \overline{y_u^{tp}} Q_{eB}^{sr} (\xi_{rp} - 1) + Q_{lequ}^{(1)srt p} \left( \right. \\
& - \frac{9}{16} g_L^2 - \frac{7}{3} g_s^2 - \frac{415}{144} g_Y^2 \left. \right) \\
& + Q_{lequ}^{(3)srt p} \left( -\frac{1}{12} g_s^2 - \frac{15}{64} g_L^2 \right. \\
& - \frac{265}{576} g_Y^2 \left. \right) - \frac{3}{32} \overline{y_e^{ur}} \overline{y_u^{vp}} Q_{lq}^{(1)sutv} - \frac{3}{8} \overline{y_e^{su}} \overline{y_u^{vp}} Q_{eu}^{urvp} \\
& \left. - \frac{3}{8} g_L \overline{y_u^{tp}} Q_{eW}^{sr} (\xi_{rp} - 1) \right]
\end{aligned} \tag{2.23}$$

$$\begin{aligned}
R_{q^c q q^c \ell}^{prst} = & -Q_{qqq}^{sprt} - Q_{qqq}^{srpt} + \frac{1}{16\pi^2} \left[ Q_{duq}^{uvpt} \left( y_d^{su} y_u^{rv} \right. \right. \\
& + y_d^{ru} y_u^{sv} \left. \right) + y_e^{tu} y_u^{sv} Q_{qqu}^{prvu} + \frac{21}{2} g_L^2 Q_{qqq}^{sprt} \\
& - y_e^{tu} y_u^{rv} Q_{qqu}^{psvu} - 2 y_d^{pu} y_u^{rv} Q_{duq}^{uvst} - \frac{7}{2} g_L^2 Q_{qqq}^{prst} \\
& \left. - 7 g_L^2 Q_{qqq}^{psrt} \right]
\end{aligned} \tag{2.24}$$

$$\begin{aligned}
R_{u^c u d^c e}^{prst} = & Q_{duu}^{srpt} - Q_{duu}^{sprt} + \frac{1}{16\pi^2} \left[ -\overline{y_e^{ut}} \overline{y_u^{vp}} Q_{duq}^{srvu} \right. \\
& \left. - \overline{y_d^{us}} \overline{y_u^{vp}} Q_{qqu}^{uvrt} - \frac{35}{3} g_Y^2 Q_{duu}^{sprt} \right]
\end{aligned} \tag{2.25}$$

$$\begin{aligned}
R_{\ell\ell}^{(3)prst} = & 2Q_{\ell\ell}^{ptsr} - Q_{\ell\ell}^{prst} + \frac{1}{16\pi^2} \left[ \frac{2}{9} g_Y^2 \delta^{st} Q_{lq}^{(1)pruu} \right. \\
& + \frac{8}{9} g_Y^2 \delta^{rs} Q_{ld}^{ptuu} + \frac{8}{9} g_Y^2 \delta^{st} Q_{lu}^{pruu} + Q_{H\ell}^{(1)pr} \left( \frac{2}{3} g_Y^2 \delta^{st} \right. \\
& + 2 \overline{y_e^{su}} y_e^{tu} \left. \right) + Q_{H\ell}^{(1)pt} \left( -\frac{4}{3} g_Y^2 \delta^{rs} \right. \\
& - 4 \overline{y_e^{su}} y_e^{ru} \left. \right) + Q_{H\ell}^{(3)pr} \left( 2 \overline{y_e^{su}} y_e^{tu} - \frac{2}{3} g_L^2 \delta^{st} \right) \\
& + Q_{\ell\ell}^{uupr} \left( \frac{2}{3} g_L^2 \delta^{st} - \frac{2}{3} g_Y^2 \delta^{st} \right) + \frac{4}{3} g_Y^2 \delta^{rs} Q_{\ell\ell}^{uupt} \\
& + 2 \overline{y_e^{su}} y_e^{tv} Q_{\ell e}^{pruv} + \frac{8}{3} g_Y^2 \delta^{rs} Q_{\ell e}^{ptuu} - \frac{4}{9} g_Y^2 \delta^{st} Q_{ld}^{pruu} \\
& - \frac{4}{9} g_Y^2 \delta^{rs} Q_{lq}^{(1)ptuu} - \frac{2}{3} g_L^2 \delta^{st} Q_{lq}^{(3)pruu} - \frac{4}{3} g_Y^2 \delta^{st} Q_{\ell e}^{pruu} \\
& \left. - \frac{4}{3} g_L^2 \delta^{st} Q_{\ell\ell}^{urpu} - \frac{16}{9} g_Y^2 \delta^{rs} Q_{lu}^{ptuu} - 4 \overline{y_e^{su}} y_e^{rv} Q_{\ell e}^{ptuv} \right]
\end{aligned} \tag{2.26}$$

$$\begin{aligned}
R_{qq}^{(1,8)prst} = & \frac{1}{4} Q_{qq}^{(1)ptsr} + \frac{1}{4} Q_{qq}^{(3)ptsr} - \frac{1}{6} Q_{qq}^{(1)prst} \\
& + \frac{1}{16\pi^2} \left[ \frac{1}{18} g_Y^2 \delta^{rs} Q_{qq}^{(1)uupt} + \frac{2}{27} g_Y^2 \delta^{st} Q_{qd}^{(1)pruu} + \frac{1}{9} g_Y^2 \delta^{st} Q_{lq}^{(1)uupr} \right.
\end{aligned} \tag{2.27}$$

$$\begin{aligned}
& + \frac{2}{9} g_Y^2 \delta^{st} Q_{qe}^{pruu} + \frac{2}{9} g_Y^2 \delta^{rs} Q_{qu}^{(1)ptuu} + \frac{1}{3} \overline{y_d^{su}} y_d^{tv} Q_{qd}^{(1)pruv} \\
& + \frac{1}{3} \overline{y_u^{su}} y_u^{tv} Q_{qu}^{(1)pruv} + \frac{1}{2} g_L^2 \delta^{rs} Q_{\ell q}^{(3)uupt} + \frac{1}{2} g_L^2 \delta^{rs} Q_{qq}^{(3)uupt} \\
& + \overline{y_d^{pu}} \overline{y_u^{sv}} \left( -\frac{1}{6} \overline{Q_{quqd}^{(1)tvr u}} - \frac{1}{2} \overline{Q_{quqd}^{(1)rvtu}} \right. \\
& \left. - \overline{Q_{quqd}^{(8)tvr u}} \right) + Q_{Hq}^{(1)pr} \left( \overline{y_d^{su}} y_d^{tu} - \frac{1}{9} g_Y^2 \delta^{st} \right. \\
& \left. - \overline{y_u^{su}} y_u^{tu} \right) + Q_{Hq}^{(1)pt} \left( \frac{1}{6} g_Y^2 \delta^{rs} + \frac{3}{2} \overline{y_u^{su}} y_u^{ru} \right. \\
& \left. - \frac{3}{2} \overline{y_d^{su}} y_d^{ru} \right) + Q_{Hq}^{(3)pt} \left( \frac{1}{2} g_L^2 \delta^{rs} - \frac{3}{2} \overline{y_d^{su}} y_d^{ru} \right. \\
& \left. - \frac{3}{2} \overline{y_u^{su}} y_u^{ru} \right) + Q_{qq}^{(1)uupr} \left( \frac{2}{9} g_s^2 \delta^{st} - \frac{1}{27} g_Y^2 \delta^{st} \right) \\
& + Q_{quqd}^{(1)pvsu} \left( -\frac{1}{6} y_d^{tu} y_u^{rv} - \frac{1}{2} y_d^{ru} y_u^{tv} \right) \\
& + 2 \overline{y_d^{su}} y_d^{tv} Q_{qd}^{(8)pruv} + 2 \overline{y_u^{su}} y_u^{tv} Q_{qu}^{(8)pruv} - \frac{1}{9} g_Y^2 \delta^{rs} Q_{qd}^{(1)ptuu} \\
& - \frac{4}{27} g_Y^2 \delta^{st} Q_{qu}^{(1)pruu} - \frac{1}{6} g_Y^2 \delta^{rs} Q_{\ell q}^{(1)uupt} - \frac{1}{3} g_Y^2 \delta^{rs} Q_{qe}^{ptuu} \\
& - \frac{1}{3} g_s^2 \delta^{st} Q_{qq}^{(1)urpu} - \frac{1}{3} g_s^2 \delta^{st} Q_{qq}^{(3)urpu} - \frac{1}{2} \overline{y_d^{su}} y_d^{rv} Q_{qd}^{(1)ptuv} \\
& - \frac{1}{2} \overline{y_u^{su}} y_u^{rv} Q_{qu}^{(1)ptuv} - y_d^{tu} y_u^{rv} Q_{quqd}^{(8)pvsu} - \frac{4}{3} g_s^2 \delta^{st} Q_{qd}^{(8)pruu} \\
& \left. - \frac{4}{3} g_s^2 \delta^{st} Q_{qu}^{(8)pruu} \right]
\end{aligned}$$

$$R_{qq}^{(3,8)prst} = \frac{3}{4} Q_{qq}^{(1)ptsr} - \frac{1}{6} Q_{qq}^{(3)prst} - \frac{1}{4} Q_{qq}^{(3)ptsr} \quad (2.28)$$

$$\begin{aligned}
& + \frac{1}{16\pi^2} \left[ \frac{1}{6} g_Y^2 \delta^{rs} Q_{qq}^{(1)uupt} + \frac{2}{3} g_Y^2 \delta^{rs} Q_{qu}^{(1)ptuu} + \overline{y_d^{pu}} \overline{y_u^{sv}} \left( \frac{1}{2} \overline{Q_{quqd}^{(1)tvr u}} \right. \right. \\
& + \frac{3}{2} \overline{Q_{quqd}^{(1)rvtu}} + 3 \overline{Q_{quqd}^{(8)tvr u}} \left. \right) + Q_{Hq}^{(1)pt} \left( \frac{1}{2} g_Y^2 \delta^{rs} \right. \\
& + \frac{9}{2} \overline{y_u^{su}} y_u^{ru} - \frac{9}{2} \overline{y_d^{su}} y_d^{ru} \left. \right) + Q_{Hq}^{(3)pr} \left( \overline{y_d^{su}} y_d^{tu} \right. \\
& + \overline{y_u^{su}} y_u^{tu} - \frac{1}{3} g_L^2 \delta^{st} \left. \right) + Q_{Hq}^{(3)pt} \left( \frac{3}{2} \overline{y_d^{su}} y_d^{ru} \right. \\
& + \frac{3}{2} \overline{y_u^{su}} y_u^{ru} - \frac{1}{2} g_L^2 \delta^{rs} \left. \right) + Q_{quqd}^{(1)pvsu} \left( \frac{1}{2} y_d^{tu} y_u^{rv} \right. \\
& + \frac{3}{2} y_d^{ru} y_u^{tv} \left. \right) + 3 y_d^{tu} y_u^{rv} Q_{quqd}^{(8)pvsu} - \frac{1}{3} g_L^2 \delta^{st} Q_{\ell q}^{(3)uupr} \\
& - \frac{1}{3} g_Y^2 \delta^{rs} Q_{qd}^{(1)ptuu} - \frac{1}{3} g_L^2 \delta^{st} Q_{qq}^{(3)uupr} - \frac{1}{2} g_Y^2 \delta^{rs} Q_{\ell q}^{(1)uupt} \\
& - \frac{1}{2} g_L^2 \delta^{rs} Q_{\ell q}^{(3)uupt} - \frac{1}{2} g_L^2 \delta^{rs} Q_{qq}^{(3)uupt} - g_Y^2 \delta^{rs} Q_{qe}^{ptuu} \\
& \left. - \frac{3}{2} \overline{y_d^{su}} y_d^{rv} Q_{qd}^{(1)ptuv} - \frac{3}{2} \overline{y_u^{su}} y_u^{rv} Q_{qu}^{(1)ptuv} \right]
\end{aligned}$$

$$R_{\ell q}^{(1)prst} = \frac{1}{2} Q_{\ell q}^{(1)ptsr} + \frac{1}{2} Q_{\ell q}^{(3)ptsr} + \frac{1}{16\pi^2} \left[ \frac{1}{18} g_Y^2 \delta^{rs} Q_{\ell q}^{(1)ptuu} \right] \quad (2.29)$$

$$\begin{aligned}
& + \frac{1}{16} y_e^{tu} y_u^{rv} Q_{\ell equ}^{(3)pusv} + \frac{1}{9} g_Y^2 \delta^{pt} Q_{qd}^{(1)sruu} + \frac{1}{6} g_Y^2 \delta^{pt} Q_{\ell q}^{(1)uusr} \\
& + \frac{1}{6} g_L^2 \delta^{pt} Q_{\ell q}^{(3)uusr} + \frac{1}{6} g_L^2 \delta^{pt} Q_{qq}^{(3)uusr} + \frac{2}{9} g_Y^2 \delta^{rs} Q_{\ell u}^{ptuu} \\
& + \frac{1}{3} g_Y^2 \delta^{pt} Q_{qe}^{sruu} + \frac{1}{2} g_L^2 \delta^{rs} Q_{\ell q}^{(3)ptuu} + \frac{3}{4} y_e^{tu} y_u^{rv} Q_{\ell equ}^{(1)pusv} \\
& + \overline{y_e^{pu}} \overline{y_u^{sv}} \left( \frac{1}{16} \overline{Q_{\ell equ}^{(3)turv}} + \frac{3}{4} \overline{Q_{\ell equ}^{(1)turv}} \right) + Q_{H\ell}^{(1)pt} \left( \frac{1}{6} g_Y^2 \delta^{rs} \right. \\
& + \frac{3}{2} \overline{y_u^{su}} y_u^{ru} - \frac{3}{2} \overline{y_d^{su}} y_d^{ru} \left. \right) + Q_{H\ell}^{(3)pt} \left( \frac{1}{2} g_L^2 \delta^{rs} \right. \\
& - \frac{3}{2} \overline{y_d^{su}} y_d^{ru} - \frac{3}{2} \overline{y_u^{su}} y_u^{ru} \left. \right) + Q_{Hq}^{(1)sr} \left( \right. \\
& - \frac{1}{6} g_Y^2 \delta^{pt} - \frac{1}{2} \overline{y_e^{pu}} y_e^{tu} \left. \right) + Q_{Hq}^{(3)sr} \left( \frac{1}{6} g_L^2 \delta^{pt} \right. \\
& - \frac{1}{2} \overline{y_e^{pu}} y_e^{tu} \left. \right) + g_L^2 \delta^{rs} Q_{\ell\ell}^{utpu} + Q_{\ell\ell}^{uupt} \left( \right. \\
& - \frac{1}{6} g_Y^2 \delta^{rs} - \frac{1}{2} g_L^2 \delta^{rs} \left. \right) - \frac{1}{18} g_Y^2 \delta^{pt} Q_{qq}^{(1)uusr} \\
& - \frac{1}{9} g_Y^2 \delta^{rs} Q_{\ell d}^{ptuu} - \frac{2}{9} g_Y^2 \delta^{pt} Q_{qu}^{(1)sruu} - \frac{1}{3} g_Y^2 \delta^{rs} Q_{\ell e}^{ptuu} \\
& - \frac{1}{2} \overline{y_d^{su}} y_d^{rv} Q_{\ell d}^{ptuv} - \frac{1}{2} \overline{y_u^{su}} y_u^{rv} Q_{\ell u}^{ptuv} - \frac{1}{2} \overline{y_e^{pu}} y_e^{tv} Q_{qe}^{sruv} \\
& \left. - 2 \overline{y_e^{pu}} y_d^{rv} \overline{Q_{\ell edq}^{tuvs}} - 2 \overline{y_d^{su}} y_e^{tv} \overline{Q_{\ell edq}^{pvur}} \right]
\end{aligned}$$

$$\begin{aligned}
R_{\ell q}^{(3)prst} = & \frac{3}{2} Q_{\ell q}^{(1)ptsr} - \frac{1}{2} Q_{\ell q}^{(3)ptsr} + \frac{1}{16\pi^2} \left[ \frac{1}{6} g_Y^2 \delta^{rs} Q_{\ell q}^{(1)ptuu} \right. \\
& + \frac{1}{3} g_Y^2 \delta^{pt} Q_{qd}^{(1)sruu} + \frac{1}{2} g_Y^2 \delta^{pt} Q_{\ell q}^{(1)uusr} + \frac{2}{3} g_Y^2 \delta^{rs} Q_{\ell u}^{ptuu} \\
& + \overline{y_e^{pu}} \overline{y_u^{sv}} \left( -\frac{3}{16} \overline{Q_{\ell equ}^{(3)turv}} - \frac{9}{4} \overline{Q_{\ell equ}^{(1)turv}} \right) \\
& + Q_{H\ell}^{(1)pt} \left( \frac{1}{2} g_Y^2 \delta^{rs} + \frac{9}{2} \overline{y_u^{su}} y_u^{ru} - \frac{9}{2} \overline{y_d^{su}} y_d^{ru} \right) \\
& + Q_{H\ell}^{(3)pt} \left( \frac{3}{2} \overline{y_d^{su}} y_d^{ru} + \frac{3}{2} \overline{y_u^{su}} y_u^{ru} - \frac{1}{2} g_L^2 \delta^{rs} \right) \\
& + Q_{Hq}^{(1)sr} \left( -\frac{1}{2} g_Y^2 \delta^{pt} - \frac{3}{2} \overline{y_e^{pu}} y_e^{tu} \right) \\
& + Q_{Hq}^{(3)sr} \left( \frac{1}{2} \overline{y_e^{pu}} y_e^{tu} - \frac{1}{6} g_L^2 \delta^{pt} \right) + Q_{\ell\ell}^{uupt} \left( \frac{1}{2} g_L^2 \delta^{rs} \right. \\
& - \frac{1}{2} g_Y^2 \delta^{rs} \left. \right) + g_Y^2 \delta^{pt} Q_{qe}^{sruu} - \frac{1}{6} g_L^2 \delta^{pt} Q_{\ell q}^{(3)uusr} \\
& - \frac{1}{6} g_Y^2 \delta^{pt} Q_{qq}^{(1)uusr} - \frac{1}{6} g_L^2 \delta^{pt} Q_{qq}^{(3)uusr} - \frac{3}{16} y_e^{tu} y_u^{rv} Q_{\ell equ}^{(3)pusv} \\
& - \frac{1}{3} g_Y^2 \delta^{rs} Q_{\ell d}^{ptuu} - \frac{1}{2} g_L^2 \delta^{rs} Q_{\ell q}^{(3)ptuu} - \frac{2}{3} g_Y^2 \delta^{pt} Q_{qu}^{(1)sruu} \\
& - g_Y^2 \delta^{rs} Q_{\ell e}^{ptuu} - g_L^2 \delta^{rs} Q_{\ell\ell}^{utpu} - \frac{3}{2} \overline{y_d^{su}} y_d^{rv} Q_{\ell d}^{ptuv} \\
& \left. - \frac{3}{2} \overline{y_u^{su}} y_u^{rv} Q_{\ell u}^{ptuv} - \frac{3}{2} \overline{y_e^{pu}} y_e^{tv} Q_{qe}^{sruv} - \frac{9}{4} y_e^{tu} y_u^{rv} Q_{\ell equ}^{(1)pusv} \right]
\end{aligned} \tag{2.30}$$

$$\begin{aligned}
R_{uu}^{(8)prst} = & \frac{1}{2}Q_{uu}^{ptsr} - \frac{1}{6}Q_{uu}^{prst} + \frac{1}{16\pi^2} \left[ \frac{4}{27}g_Y^2\delta^{pr}Q_{ud}^{(1)stuu} \right. \\
& + \frac{1}{6}\overline{y_u^{ut}}y_u^{vs}Q_{qu}^{(1)vupr} + \frac{2}{9}g_Y^2\delta^{st}Q_{\ell u}^{uupr} + \frac{2}{9}g_Y^2\delta^{rs}Q_{qu}^{(1)uupt} \\
& + \frac{4}{9}g_Y^2\delta^{st}Q_{eu}^{uupr} + \frac{8}{9}g_Y^2\delta^{rs}Q_{uu}^{uupt} + Q_{Hu}^{pr}\left(\overline{y_u^{ut}}y_u^{us} \right. \\
& \left. - \frac{2}{9}g_Y^2\delta^{st}\right) + Q_{Hu}^{pt}\left(\frac{2}{3}g_Y^2\delta^{rs} - 3\overline{y_u^{ur}}y_u^{us}\right) \\
& + \overline{y_u^{ut}}y_u^{vs}Q_{qu}^{(8)vupr} + Q_{uu}^{uust}\left(\frac{1}{9}g_s^2\delta^{pr} - \frac{8}{27}g_Y^2\delta^{pr}\right) \\
& - \frac{2}{27}g_Y^2\delta^{st}Q_{qu}^{(1)uupr} - \frac{1}{3}g_s^2\delta^{pr}Q_{uu}^{utsu} - \frac{4}{9}g_Y^2\delta^{rs}Q_{ud}^{(1)ptuu} \\
& - \frac{1}{2}\overline{y_u^{ur}}y_u^{vs}Q_{qu}^{(1)vupt} - \frac{2}{3}g_Y^2\delta^{rs}Q_{\ell u}^{uupt} - \frac{2}{3}g_s^2\delta^{st}Q_{qu}^{(8)uupr} \\
& \left. - \frac{2}{3}g_s^2\delta^{pr}Q_{ud}^{(8)stuu} - \frac{4}{3}g_Y^2\delta^{rs}Q_{eu}^{uupt} \right]
\end{aligned} \tag{2.31}$$

$$\begin{aligned}
R_{dd}^{(8)prst} = & \frac{1}{2}Q_{dd}^{ptsr} - \frac{1}{6}Q_{dd}^{prst} + \frac{1}{16\pi^2} \left[ \frac{1}{27}g_Y^2\delta^{st}Q_{qd}^{(1)uupr} \right. \\
& + \frac{4}{27}g_Y^2\delta^{pr}Q_{ud}^{(1)uust} + \frac{1}{6}\overline{y_d^{ut}}y_d^{vs}Q_{qd}^{(1)vupr} + \frac{2}{9}g_Y^2\delta^{rs}Q_{dd}^{uupt} \\
& + \frac{1}{3}g_Y^2\delta^{rs}Q_{\ell d}^{uupt} + \frac{2}{3}g_Y^2\delta^{rs}Q_{ed}^{uupt} + Q_{dd}^{uupr}\left(\frac{1}{9}g_s^2\delta^{st} \right. \\
& \left. - \frac{2}{27}g_Y^2\delta^{st}\right) + Q_{Hd}^{pr}\left(\frac{1}{9}g_Y^2\delta^{st} - \overline{y_d^{ut}}y_d^{us}\right) \\
& + Q_{Hd}^{pt}\left(3\overline{y_d^{ur}}y_d^{us} - \frac{1}{3}g_Y^2\delta^{rs}\right) + \overline{y_d^{ut}}y_d^{vs}Q_{qd}^{(8)vupr} \\
& - \frac{1}{9}g_Y^2\delta^{st}Q_{\ell d}^{uupr} - \frac{1}{9}g_Y^2\delta^{rs}Q_{qd}^{(1)uupt} - \frac{2}{9}g_Y^2\delta^{st}Q_{ed}^{uupr} \\
& - \frac{1}{3}g_s^2\delta^{st}Q_{dd}^{urpu} - \frac{4}{9}g_Y^2\delta^{rs}Q_{ud}^{(1)uupt} - \frac{1}{2}\overline{y_d^{ur}}y_d^{vs}Q_{qd}^{(1)vupt} \\
& \left. - \frac{2}{3}g_s^2\delta^{st}Q_{qd}^{(8)uupr} - \frac{2}{3}g_s^2\delta^{pr}Q_{ud}^{(8)uust} \right]
\end{aligned} \tag{2.32}$$

$$\begin{aligned}
R_{eu}^{prst} = & Q_{eu}^{ptsr} + \frac{1}{16\pi^2} \left[ \frac{2}{9}g_Y^2\delta^{rs}Q_{qe}^{uupt} + \frac{2}{9}g_Y^2\delta^{pt}Q_{ud}^{(1)sruu} \right. \\
& + \frac{1}{3}g_Y^2\delta^{pt}Q_{\ell u}^{uusr} + \frac{2}{3}g_Y^2\delta^{pt}Q_{eu}^{uusr} + \frac{8}{9}g_Y^2\delta^{rs}Q_{eu}^{ptuu} \\
& + \overline{y_e^{ut}}\overline{y_u^{vr}}\left(-\frac{1}{16}Q_{\ell equ}^{(3)upvs} - \frac{3}{4}Q_{\ell equ}^{(1)upvs}\right) \\
& + Q_{He}^{pt}\left(\frac{2}{3}g_Y^2\delta^{rs} - 3\overline{y_u^{ur}}y_u^{us}\right) + Q_{Hu}^{sr}\left(\overline{y_e^{ut}}y_e^{up} \right. \\
& \left. - \frac{1}{3}g_Y^2\delta^{pt}\right) - \frac{1}{16}y_e^{up}y_u^{vs}Q_{\ell equ}^{(3)utvr} - \frac{1}{9}g_Y^2\delta^{pt}Q_{qu}^{(1)uusr} \\
& - \frac{4}{9}g_Y^2\delta^{rs}Q_{ed}^{ptuu} - \frac{4}{9}g_Y^2\delta^{pt}Q_{uu}^{uusr} - \frac{1}{2}\overline{y_e^{ut}}y_e^{vp}Q_{\ell u}^{vusr} \\
& \left. - \frac{1}{2}\overline{y_u^{ur}}y_u^{vs}Q_{qe}^{vupt} - \frac{2}{3}g_Y^2\delta^{rs}Q_{\ell e}^{uupt} - \frac{3}{4}y_e^{up}y_u^{vs}Q_{\ell equ}^{(1)utvr} \right]
\end{aligned} \tag{2.33}$$

$$\begin{aligned}
& -\frac{4}{3}g_Y^2\delta^{rs}Q_{ee}^{ptuu}\Big] \\
R_{ed}^{prst} = & Q_{ed}^{ptsr} + \frac{1}{16\pi^2}\Bigg[\frac{2}{9}g_Y^2\delta^{pt}Q_{dd}^{uusr} + \frac{2}{9}g_Y^2\delta^{rs}Q_{ed}^{ptuu} \\
& + \frac{1}{3}g_Y^2\delta^{pt}Q_{ld}^{uusr} + \frac{1}{3}g_Y^2\delta^{rs}Q_{le}^{uupt} + \frac{2}{3}g_Y^2\delta^{pt}Q_{ed}^{uusr} \\
& + \frac{2}{3}g_Y^2\delta^{rs}Q_{ee}^{ptuu} + Q_{Hd}^{sr}\left(\overline{y_e^{ut}}y_e^{up} - \frac{1}{3}g_Y^2\delta^{pt}\right) \\
& + Q_{He}^{pt}\left(3\overline{y_d^{ur}}y_d^{us} - \frac{1}{3}g_Y^2\delta^{rs}\right) - \frac{1}{9}g_Y^2\delta^{pt}Q_{qd}^{(1)uusr} \\
& - \frac{1}{9}g_Y^2\delta^{rs}Q_{qe}^{uupt} - \frac{4}{9}g_Y^2\delta^{rs}Q_{eu}^{ptuu} - \frac{4}{9}g_Y^2\delta^{pt}Q_{ud}^{(1)uusr} \\
& - \frac{1}{2}\overline{y_e^{ut}}y_e^{vp}Q_{ld}^{vusr} - \frac{1}{2}\overline{y_d^{ur}}y_d^{vs}Q_{qe}^{vupt} - \overline{y_e^{ut}}y_d^{vs}Q_{ledq}^{\overline{uprv}} \\
& - \overline{y_d^{ur}}y_e^{vp}Q_{ledq}^{vtsu}\Big]
\end{aligned} \tag{2.34}$$

$$\begin{aligned}
R_{ud}^{(1)prst} = & \frac{1}{3}Q_{ud}^{(1)ptsr} + 2Q_{ud}^{(8)ptsr} + \frac{1}{16\pi^2}\Bigg[\frac{2}{27}g_Y^2\delta^{pt}Q_{qd}^{(1)uusr} \\
& + \frac{2}{27}g_Y^2\delta^{rs}Q_{ud}^{(1)ptuu} + \frac{1}{9}g_Y^2\delta^{rs}Q_{lu}^{uupt} + \frac{1}{6}y_d^{us}y_u^{vp}Q_{quqd}^{(1)vtur} \\
& + \frac{2}{9}g_Y^2\delta^{rs}Q_{eu}^{uupt} + \frac{8}{27}g_Y^2\delta^{pt}Q_{ud}^{(1)uusr} + \frac{1}{3}g_s^2\delta^{pt}Q_{dd}^{ursu} \\
& + \frac{1}{3}g_s^2\delta^{rs}Q_{uu}^{utpu} + \frac{1}{2}y_d^{us}y_u^{vp}Q_{quqd}^{(1)utvr} + \frac{2}{3}g_s^2\delta^{pt}Q_{qd}^{(8)uusr} \\
& + \frac{2}{3}g_s^2\delta^{rs}Q_{qu}^{(8)uupt} + \frac{2}{3}g_s^2\delta^{rs}Q_{ud}^{(8)ptuu} + \frac{2}{3}g_s^2\delta^{pt}Q_{ud}^{(8)uusr} \\
& + \overline{y_d^{ur}}\overline{y_u^{vt}}\left(\frac{1}{6}Q_{quqd}^{(1)vpus} + \frac{1}{2}Q_{quqd}^{(1)upvs} + Q_{quqd}^{(8)vpus}\right) \\
& + Q_{dd}^{uusr}\left(-\frac{1}{9}g_s^2\delta^{pt} - \frac{4}{27}g_Y^2\delta^{pt}\right) \\
& + Q_{Hd}^{sr}\left(\frac{2}{9}g_Y^2\delta^{pt} - \overline{y_u^{ut}}y_u^{up}\right) + Q_{Hu}^{pt}\left(\overline{y_d^{ur}}y_d^{us} - \frac{1}{9}g_Y^2\delta^{rs}\right) \\
& + y_d^{us}y_u^{vp}Q_{quqd}^{(8)vtur} + Q_{uu}^{uupt}\left(-\frac{1}{9}g_s^2\delta^{rs} - \frac{4}{27}g_Y^2\delta^{rs}\right) - \frac{1}{27}g_Y^2\delta^{rs}Q_{qu}^{(1)uupt} \\
& - \frac{1}{6}\overline{y_u^{ut}}y_u^{vp}Q_{qd}^{(1)vusr} - \frac{1}{6}\overline{y_d^{ur}}y_d^{vs}Q_{qu}^{(1)vupt} - \frac{2}{9}g_Y^2\delta^{pt}Q_{ld}^{uusr} \\
& - \frac{4}{9}g_Y^2\delta^{pt}Q_{ed}^{uusr} - \overline{y_u^{ut}}y_u^{vp}Q_{qd}^{(8)vusr} - \overline{y_d^{ur}}y_d^{vs}Q_{qu}^{(8)vupt} \\
& - 6\overline{y_d^{ur}}y_u^{up}Q_{Hud}^{ts} - 6\overline{y_u^{ut}}y_d^{us}Q_{Hud}^{pr}\Big]
\end{aligned} \tag{2.35}$$

$$\begin{aligned}
R_{ud}^{(8)prst} = & \frac{4}{9}Q_{ud}^{(1)ptsr} - \frac{1}{3}Q_{ud}^{(8)ptsr} + \frac{1}{16\pi^2}\Bigg[\frac{8}{81}g_Y^2\delta^{pt}Q_{qd}^{(1)uusr} \\
& + \frac{8}{81}g_Y^2\delta^{rs}Q_{ud}^{(1)ptuu} + \frac{4}{27}g_Y^2\delta^{rs}Q_{lu}^{uupt} + \frac{1}{6}\overline{y_u^{ut}}y_u^{vp}Q_{qd}^{(8)vusr}
\end{aligned} \tag{2.36}$$

$$\begin{aligned}
& + \frac{1}{6} \overline{y_d^{ur}} y_d^{vs} Q_{qu}^{(8)vupt} + \frac{2}{9} y_d^{us} y_u^{vp} Q_{quqd}^{(1)vtur} + \frac{8}{27} g_Y^2 \delta^{rs} Q_{eu}^{uupt} \\
& + \frac{32}{81} g_Y^2 \delta^{pt} Q_{ud}^{(1)uusr} + \frac{1}{2} y_d^{us} y_u^{vp} Q_{quqd}^{(8)utvr} + \overline{y_d^{ur}} \overline{y_u^{vt}} \left( \frac{2}{9} \overline{Q_{quqd}^{(1)vpus}} \right. \\
& + \frac{1}{2} \overline{Q_{quqd}^{(8)upvs}} - \frac{1}{6} \overline{Q_{quqd}^{(8)vpus}} \left. \right) + Q_{dd}^{uusr} \left( \frac{1}{54} g_s^2 \delta^{pt} \right. \\
& - \frac{16}{81} g_Y^2 \delta^{pt} \left. \right) + Q_{Hd}^{sr} \left( \frac{8}{27} g_Y^2 \delta^{pt} - \frac{4}{3} \overline{y_u^{ut}} y_u^{up} \right) \\
& + Q_{Hu}^{pt} \left( \frac{4}{3} \overline{y_d^{ur}} y_d^{us} - \frac{4}{27} g_Y^2 \delta^{rs} \right) + Q_{uu}^{uupt} \left( \frac{1}{54} g_s^2 \delta^{rs} \right. \\
& - \frac{16}{81} g_Y^2 \delta^{rs} \left. \right) - \frac{4}{81} g_Y^2 \delta^{rs} Q_{qu}^{(1)uupt} - \frac{1}{18} g_s^2 \delta^{pt} Q_{dd}^{ursu} \\
& - \frac{1}{18} g_s^2 \delta^{rs} Q_{uu}^{utpu} - \frac{1}{9} g_s^2 \delta^{pt} Q_{qd}^{(8)uusr} - \frac{1}{9} g_s^2 \delta^{rs} Q_{qu}^{(8)uupt} \\
& - \frac{1}{9} g_s^2 \delta^{rs} Q_{ud}^{(8)ptuu} - \frac{1}{9} g_s^2 \delta^{pt} Q_{ud}^{(8)uusr} - \frac{1}{6} y_d^{us} y_u^{vp} Q_{quqd}^{(8)vtur} \\
& - \frac{2}{9} \overline{y_u^{ut}} y_u^{vp} Q_{qd}^{(1)vusr} - \frac{2}{9} \overline{y_d^{ur}} y_d^{vs} Q_{qu}^{(1)vupt} - \frac{8}{27} g_Y^2 \delta^{pt} Q_{ld}^{uusr} \\
& - \left. \frac{16}{27} g_Y^2 \delta^{pt} Q_{ed}^{uusr} \right]
\end{aligned}$$

$$R_{\ell qde}^{prst} = -2Q_{\ell edq}^{ptsr} + \frac{1}{16\pi^2} \left[ \frac{1}{6} \overline{y_e^{pt}} y_d^{uv} Q_{qd}^{(1)ursv} + \frac{1}{4} g_Y y_d^{rs} Q_{eB}^{pt} \right. \quad (2.37)$$

$$\begin{aligned}
& + \frac{3}{4} g_Y \overline{y_e^{pt}} \overline{Q_{dB}^{rs}} + Q_{eH}^{pt} \left( 6 \overline{y_d^{uv}} y_d^{rv} y_d^{us} - 3 \lambda y_d^{rs} \right) \\
& + Q_{\ell equ}^{(1)ptuv} \left( \frac{3}{4} y_d^{us} y_u^{rv} + 3 y_d^{rs} y_u^{uv} \right) + \overline{y_e^{pt}} y_d^{uv} Q_{qd}^{(8)ursv} \\
& + \frac{3}{2} \overline{y_e^{uv}} y_d^{rs} Q_{\ell e}^{puvt} + 2 \overline{y_e^{pu}} \overline{y_e^{vt}} y_e^{vu} \overline{Q_{dH}^{rs}} - \frac{1}{16} y_d^{us} y_u^{rv} Q_{\ell equ}^{(3)ptuv} \\
& - \frac{1}{4} g_L \overline{y_e^{pt}} \overline{Q_{dW}^{rs}} - \frac{1}{4} \overline{y_e^{ut}} y_d^{vs} Q_{\ell q}^{(1)puvr} - \frac{1}{4} \overline{y_e^{ut}} y_d^{vs} Q_{\ell q}^{(3)puvr} \\
& - \frac{1}{2} \overline{y_e^{ut}} y_d^{rv} Q_{\ell d}^{pusv} - \frac{1}{2} \overline{y_e^{pu}} y_d^{vs} Q_{qe}^{vnut} - \frac{3}{4} g_L y_d^{rs} Q_{eW}^{pt} \\
& - \overline{y_e^{pt}} \overline{y_u^{uv}} \overline{Q_{quqd}^{(1)uvrs}} - \lambda \overline{y_e^{pt}} \overline{Q_{dH}^{rs}} - \mu^2 \overline{y_e^{pt}} \overline{Q_{yd}^{rs}} \\
& - \overline{y_e^{pu}} y_d^{rv} Q_{ed}^{utsv} - \overline{y_e^{pt}} y_e^{uv} Q_{\ell edq}^{uvsr} - 3 \overline{y_d^{uv}} y_d^{rs} Q_{\ell edq}^{ptvu} \\
& - \left. 3 \mu^2 y_d^{rs} Q_{ye}^{pt} \right]
\end{aligned}$$

$$R_{\ell ce}^{prst} = -Q_{\ell e}^{tpsr} + \frac{1}{16\pi^2} \left[ \frac{1}{9} g_Y^2 \delta^{rs} Q_{\ell q}^{(1)tpuu} + \frac{1}{9} g_Y^2 \delta^{pt} Q_{qe}^{uusr} \right. \quad (2.38)$$

$$\begin{aligned}
& + \frac{4}{9} g_Y^2 \delta^{pt} Q_{eu}^{sruu} + \frac{4}{9} g_Y^2 \delta^{rs} Q_{\ell u}^{tpuu} + \frac{1}{2} \overline{y_e^{ur}} y_e^{vs} Q_{\ell \ell}^{vutp} \\
& + \overline{y_e^{tu}} y_e^{pv} Q_{ee}^{uvsr} + Q_{He}^{sr} \left( \frac{1}{3} g_Y^2 \delta^{pt} + \overline{y_e^{tu}} y_e^{pu} \right) \\
& + Q_{H\ell}^{(1)tp} \left( \frac{1}{3} g_Y^2 \delta^{rs} - \overline{y_e^{ur}} y_e^{us} \right) + Q_{\ell e}^{tpsr} \left( \right. \\
& - \frac{9}{4} g_L^2 - \frac{27}{4} g_Y^2 \left. \right) + \frac{3}{2} g_Y \overline{y_e^{tr}} \overline{Q_{eB}^{ps}}
\end{aligned}$$

$$\begin{aligned}
& + \frac{3}{2} g_Y y_e^{ps} Q_{eB}^{tr} - \frac{2}{9} g_Y^2 \delta^{pt} Q_{ed}^{sr uu} - \frac{2}{9} g_Y^2 \delta^{rs} Q_{ld}^{tp uu} \\
& - \frac{1}{3} g_Y^2 \delta^{pt} Q_{le}^{uusr} - \frac{1}{3} g_Y^2 \delta^{rs} Q_{\ell\ell}^{uutp} - \frac{1}{2} g_L \overline{y_e^{tr}} \overline{Q_{eW}^{ps}} \\
& - \frac{1}{2} g_L y_e^{ps} Q_{eW}^{tr} - \frac{2}{3} g_Y^2 \delta^{pt} Q_{ee}^{sr uu} - \frac{2}{3} g_Y^2 \delta^{rs} Q_{le}^{tp uu} \\
& - \overline{y_e^{ur}} y_e^{pv} Q_{le}^{tusv} - \overline{y_e^{tu}} y_e^{vs} Q_{le}^{vpur} \Big]
\end{aligned}$$

$$\begin{aligned}
R_{\ell^c u}^{prst} = & -Q_{\ell u}^{tpsr} + \frac{1}{16\pi^2} \left[ \frac{1}{16} y_e^{pu} y_u^{vs} Q_{lequ}^{(3)tu vr} + \frac{1}{9} g_Y^2 \delta^{pt} Q_{qu}^{(1)uusr} \right. \\
& + \frac{4}{9} g_Y^2 \delta^{rs} Q_{ld}^{tp uu} + \frac{4}{9} g_Y^2 \delta^{pt} Q_{uu}^{uusr} + \frac{2}{3} g_Y^2 \delta^{rs} Q_{\ell\ell}^{uutp} \\
& + \overline{y_e^{tu}} \overline{y_u^{vr}} \left( \frac{1}{16} \overline{Q_{lequ}^{(3)puvs}} - \frac{3}{4} \overline{Q_{lequ}^{(1)puvs}} \right) + Q_{H\ell}^{(1)tp} \left( 3 \overline{y_u^{ur}} y_u^{us} \right. \\
& - \frac{2}{3} g_Y^2 \delta^{rs} \Big) + Q_{Hu}^{sr} \left( \frac{1}{3} g_Y^2 \delta^{pt} + \overline{y_e^{tu}} y_e^{pu} \right) \\
& + Q_{\ell u}^{tpsr} \left( -\frac{1}{12} g_Y^2 - \frac{9}{4} g_L^2 \right. \\
& - 4g_s^2 \Big) + \frac{4}{3} g_Y^2 \delta^{rs} Q_{le}^{tp uu} - \frac{2}{9} g_Y^2 \delta^{rs} Q_{\ell q}^{(1)tp uu} \\
& - \frac{2}{9} g_Y^2 \delta^{pt} Q_{ud}^{(1)sr uu} - \frac{1}{3} g_Y^2 \delta^{pt} Q_{\ell u}^{uusr} - \frac{2}{3} g_Y^2 \delta^{pt} Q_{eu}^{uusr} \\
& - \frac{3}{4} y_e^{pu} y_u^{vs} Q_{lequ}^{(1)tu vr} - \frac{8}{9} g_Y^2 \delta^{rs} Q_{\ell u}^{tp uu} - \overline{y_u^{ur}} y_u^{vs} Q_{\ell q}^{(1)tp vu} \\
& \left. - 2 \overline{y_e^{tu}} y_e^{pv} Q_{eu}^{uvsr} \right]
\end{aligned} \tag{2.39}$$

$$\begin{aligned}
R_{\ell^c d}^{prst} = & -Q_{\ell d}^{tpsr} + \frac{1}{16\pi^2} \left[ \frac{1}{9} g_Y^2 \delta^{rs} Q_{\ell q}^{(1)tp uu} + \frac{1}{9} g_Y^2 \delta^{pt} Q_{qd}^{(1)uusr} \right. \\
& + \frac{4}{9} g_Y^2 \delta^{rs} Q_{\ell u}^{tp uu} + \frac{4}{9} g_Y^2 \delta^{pt} Q_{ud}^{(1)uusr} + Q_{Hd}^{sr} \left( \frac{1}{3} g_Y^2 \delta^{pt} \right. \\
& + \overline{y_e^{tu}} y_e^{pu} \Big) + Q_{H\ell}^{(1)tp} \left( \frac{1}{3} g_Y^2 \delta^{rs} - 3 \overline{y_d^{ur}} y_d^{us} \right) \\
& + Q_{\ell d}^{tpsr} \left( -\frac{25}{12} g_Y^2 - \frac{9}{4} g_L^2 \right. \\
& - 4g_s^2 \Big) + 2 \overline{y_e^{tu}} y_d^{vs} \overline{Q_{ledq}^{purv}} + 2 \overline{y_d^{ur}} y_e^{pv} Q_{ledq}^{tvsu} \\
& - \frac{2}{9} g_Y^2 \delta^{pt} Q_{dd}^{uusr} - \frac{2}{9} g_Y^2 \delta^{rs} Q_{\ell d}^{tp uu} - \frac{1}{3} g_Y^2 \delta^{pt} Q_{\ell d}^{uusr} \\
& - \frac{1}{3} g_Y^2 \delta^{rs} Q_{\ell\ell}^{uutp} - \frac{2}{3} g_Y^2 \delta^{pt} Q_{ed}^{uusr} - \frac{2}{3} g_Y^2 \delta^{rs} Q_{le}^{tp uu} \\
& \left. - \overline{y_d^{ur}} y_d^{vs} Q_{\ell q}^{(1)tp vu} - 2 \overline{y_e^{tu}} y_e^{pv} Q_{ed}^{uvsr} \right]
\end{aligned} \tag{2.40}$$

$$\begin{aligned}
R_{q^c ed \ell^c}^{prst} = & 2Q_{ledq}^{trsp} + \frac{1}{16\pi^2} \left[ \frac{1}{4} g_Y y_d^{ps} Q_{eB}^{tr} + \frac{1}{2} \overline{y_e^{ur}} y_d^{vs} Q_{\ell q}^{(1)tu vp} \right. \\
& + \frac{1}{2} \overline{y_e^{ur}} y_d^{vs} Q_{\ell q}^{(3)tu vp} + \frac{3}{4} g_Y \overline{y_e^{tr}} \overline{Q_{dB}^{ps}} + \overline{y_e^{tr}} \overline{y_u^{uv}} \overline{Q_{quqd}^{(1)uvps}} \Big]
\end{aligned} \tag{2.41}$$



$$\begin{aligned}
& + \lambda \overline{y_e^{tr}} \overline{Q_{dH}^{ps}} + \mu^2 \overline{y_e^{tr}} \overline{Q_{yd}^{ps}} + Q_{eH}^{tr} \left( 3\lambda y_d^{ps} \right. \\
& - 6\overline{y_d^{uv}} y_d^{pv} y_d^{us} \left. \right) + Q_{ledq}^{trsp} \left( \frac{3}{2} g_Y^2 + \frac{9}{2} g_L^2 \right) \\
& + \overline{y_e^{tr}} y_e^{uv} Q_{ledq}^{uvsp} + Q_{lequ}^{(1)truv} \left( -\frac{3}{4} y_d^{us} y_u^{pv} \right. \\
& - 3y_d^{ps} y_u^{uv} \left. \right) + 2\overline{y_e^{tu}} y_d^{pv} Q_{ed}^{ursv} + 3\overline{y_d^{uv}} y_d^{ps} Q_{ledq}^{trvu} \\
& + 3\mu^2 y_d^{ps} Q_{ye}^{tr} - \frac{1}{16} y_d^{us} y_u^{pv} Q_{lequ}^{(3)truv} - \frac{1}{6} \overline{y_e^{tr}} y_d^{uv} Q_{qd}^{(1)upsv} \\
& - \frac{1}{4} g_L \overline{y_e^{tr}} \overline{Q_{dW}^{ps}} - \frac{1}{2} \overline{y_e^{ur}} y_d^{pv} Q_{ld}^{tusv} - \frac{1}{2} \overline{y_e^{tu}} y_d^{vs} Q_{qe}^{vpur} \\
& - \frac{3}{4} g_L y_d^{ps} Q_{eW}^{tr} - \overline{y_e^{tr}} y_d^{uv} Q_{qd}^{(8)upsv} - \frac{3}{2} \overline{y_e^{uv}} y_d^{ps} Q_{le}^{tuvr} \\
& \left. - 2\overline{y_e^{tu}} \overline{y_e^{vr}} y_e^{vu} \overline{Q_{dH}^{ps}} \right]
\end{aligned}$$

$$\begin{aligned}
R_{q^c e}^{prst} = & -Q_{qe}^{tpsr} + \frac{1}{16\pi^2} \left[ \frac{1}{16} y_e^{us} y_u^{pv} Q_{lequ}^{(3)urtv} + \frac{1}{9} g_Y^2 \delta^{rs} Q_{qq}^{(1)uutp} \right. \\
& + \frac{2}{9} g_Y^2 \delta^{pt} Q_{ed}^{sruu} + \frac{1}{3} g_Y^2 \delta^{pt} Q_{le}^{uusr} + \frac{4}{9} g_Y^2 \delta^{rs} Q_{qu}^{(1)tpuu} \\
& + \frac{2}{3} g_Y^2 \delta^{pt} Q_{ee}^{sruu} + \overline{y_e^{ur}} \overline{y_u^{tv}} \left( \frac{1}{16} \overline{Q_{lequ}^{(3)uspv}} - \frac{3}{4} \overline{Q_{lequ}^{(1)uspv}} \right) \\
& + Q_{He}^{sr} \left( 3\overline{y_d^{tu}} y_d^{pu} - \frac{1}{3} g_Y^2 \delta^{pt} - 3\overline{y_u^{tu}} y_u^{pu} \right) \\
& + Q_{Hq}^{(1)tp} \left( \frac{1}{3} g_Y^2 \delta^{rs} - \overline{y_e^{ur}} y_e^{us} \right) + Q_{qe}^{tpsr} \left( \right. \\
& - \frac{25}{12} g_Y^2 - \frac{9}{4} g_L^2 - 4g_s^2 \left. \right) \\
& + 2\overline{y_e^{ur}} y_d^{pv} \overline{Q_{ledq}^{usvt}} + 2\overline{y_d^{tu}} y_e^{vs} Q_{ledq}^{vrup} - \frac{1}{9} g_Y^2 \delta^{pt} Q_{qe}^{uusr} \\
& - \frac{2}{9} g_Y^2 \delta^{rs} Q_{qd}^{(1)tpuu} - \frac{1}{3} g_Y^2 \delta^{rs} Q_{lq}^{(1)uutp} - \frac{4}{9} g_Y^2 \delta^{pt} Q_{eu}^{sruu} \\
& - \frac{2}{3} g_Y^2 \delta^{rs} Q_{qe}^{tpuu} - \frac{3}{4} y_e^{us} y_u^{pv} Q_{lequ}^{(1)urtv} - \overline{y_e^{ur}} y_e^{vs} Q_{lq}^{(1)vutp} \\
& \left. - 2\overline{y_d^{tu}} y_d^{pv} Q_{ed}^{sruv} - 2\overline{y_u^{tu}} y_u^{pv} Q_{eu}^{sruv} \right]
\end{aligned} \tag{2.42}$$

$$\begin{aligned}
R_{q^c u}^{prst} = & -Q_{qu}^{(1)tpsr} + \frac{1}{16\pi^2} \left[ \frac{2}{9} g_Y^2 \delta^{pt} Q_{ud}^{(1)sruu} + \frac{1}{3} g_Y^2 \delta^{pt} Q_{lu}^{uusr} \right. \\
& + \frac{4}{9} g_Y^2 \delta^{rs} Q_{qd}^{(1)tpuu} + \frac{1}{2} \overline{y_u^{ur}} y_u^{vs} Q_{qq}^{(1)vutp} + \frac{2}{3} g_Y^2 \delta^{pt} Q_{eu}^{uusr} \\
& + \frac{2}{3} g_Y^2 \delta^{rs} Q_{lq}^{(1)uutp} + \overline{y_d^{tu}} \overline{y_u^{vr}} \left( \overline{Q_{quqd}^{(1)vspu}} - \frac{1}{6} \overline{Q_{quqd}^{(1)psvu}} \right. \\
& \left. - \overline{Q_{quqd}^{(8)psvu}} \right) + Q_{Hq}^{(1)tp} \left( 3\overline{y_u^{ur}} y_u^{us} - \frac{2}{3} g_Y^2 \delta^{rs} \right) \\
& + Q_{Hu}^{sr} \left( 3\overline{y_d^{tu}} y_d^{pu} - \frac{1}{3} g_Y^2 \delta^{pt} - 3\overline{y_u^{tu}} y_u^{pu} \right) \\
& \left. + Q_{qu}^{(1)tpsr} \left( -\frac{25}{12} g_Y^2 - \frac{9}{4} g_L^2 \right) \right]
\end{aligned} \tag{2.43}$$

$$\begin{aligned}
& -8g_s^2) + y_d^{pu} y_u^{vs} Q_{quqd}^{(1)vrtu} + \overline{y_u^{tu}} y_u^{pv} Q_{uu}^{uvsr} \\
& + \frac{4}{3} g_Y^2 \delta^{rs} Q_{qe}^{tpuu} - \frac{1}{9} g_Y^2 \delta^{pt} Q_{qu}^{(1)uusr} - \frac{1}{6} y_d^{pu} y_u^{vs} Q_{quqd}^{(1)trvu} \\
& - \frac{2}{9} g_Y^2 \delta^{rs} Q_{qq}^{(1)uutp} - \frac{1}{3} \overline{y_u^{ur}} y_u^{pv} Q_{qu}^{(1)tusv} - \frac{1}{3} \overline{y_u^{tu}} y_u^{vs} Q_{qu}^{(1)vpur} \\
& - \frac{4}{9} g_Y^2 \delta^{pt} Q_{uu}^{uusr} - \frac{1}{2} g_L \overline{y_u^{tr}} \overline{Q_{uW}^{ps}} - \frac{1}{2} g_L y_u^{ps} Q_{uW}^{tr} \\
& - \frac{5}{6} g_Y \overline{y_u^{tr}} \overline{Q_{uB}^{ps}} - \frac{5}{6} g_Y y_u^{ps} Q_{uB}^{tr} - \frac{8}{9} g_Y^2 \delta^{rs} Q_{qu}^{(1)tpuu} \\
& - y_d^{pu} y_u^{vs} Q_{quqd}^{(8)trvu} - 2g_s \overline{y_u^{tr}} \overline{Q_{uG}^{ps}} - 2\overline{y_u^{ur}} y_u^{pv} Q_{qu}^{(8)tusv} \\
& - 2\overline{y_u^{tu}} y_u^{vs} Q_{qu}^{(8)vpur} - 2\overline{y_d^{tu}} y_d^{pv} Q_{ud}^{(1)sruv} - 2g_s y_u^{ps} Q_{uG}^{tr} \\
& - 6g_s^2 Q_{qu}^{(8)tpsr} \Big]
\end{aligned}$$

$$\begin{aligned}
R_{q^c u}^{prst} = & -\frac{1}{3} Q_{qu}^{(1)tpsr} - 2Q_{qu}^{(8)tpsr} + \frac{1}{16\pi^2} \Bigg[ \frac{2}{27} g_Y^2 \delta^{pt} Q_{ud}^{(1)sruu} \\
& + \frac{1}{9} g_Y^2 \delta^{pt} Q_{\ell u}^{uusr} + \frac{4}{27} g_Y^2 \delta^{rs} Q_{qd}^{(1)tpuu} + \frac{2}{9} g_Y^2 \delta^{pt} Q_{eu}^{uusr} \\
& + \frac{2}{9} g_Y^2 \delta^{rs} Q_{\ell q}^{(1)uutp} + \frac{1}{4} \overline{y_u^{ur}} y_u^{vs} Q_{qq}^{(1)vptu} + \frac{1}{4} \overline{y_u^{ur}} y_u^{vs} Q_{qq}^{(3)vptu} \\
& + \frac{1}{3} y_d^{pu} y_u^{vs} Q_{quqd}^{(1)vrtu} + \frac{4}{9} g_Y^2 \delta^{rs} Q_{qe}^{tpuu} + \overline{y_d^{tu}} \overline{y_u^{vr}} \left( \frac{1}{3} \overline{Q_{quqd}^{(1)vspu}} \right. \\
& + 2\overline{Q_{quqd}^{(8)vspu}} - \left. \frac{1}{2} \overline{Q_{quqd}^{(1)psvu}} \right) + Q_{Hq}^{(1)tp} \left( \overline{y_u^{ur}} y_u^{us} \right. \\
& - \left. \frac{2}{9} g_Y^2 \delta^{rs} \right) + Q_{Hu}^{sr} \left( \overline{y_d^{tu}} y_d^{pu} - \frac{1}{9} g_Y^2 \delta^{pt} \right. \\
& - \left. \overline{y_u^{tu}} y_u^{pu} \right) + Q_{qq}^{(1)uutp} \left( \frac{1}{9} g_s^2 \delta^{rs} - \frac{2}{27} g_Y^2 \delta^{rs} \right) \\
& + Q_{qu}^{(1)tpsr} \left( -\frac{25}{36} g_Y^2 - \frac{3}{4} g_L^2 \right. \\
& - \left. \frac{16}{3} g_s^2 \right) + Q_{qu}^{(8)tpsr} \left( 4g_s^2 - \frac{25}{6} g_Y^2 \right. \\
& - \left. \frac{9}{2} g_L^2 \right) + \overline{y_u^{tu}} y_u^{pv} Q_{uu}^{ursv} + Q_{uu}^{uusr} \left( \frac{2}{9} g_s^2 \delta^{pt} \right. \\
& - \left. \frac{4}{27} g_Y^2 \delta^{pt} \right) + 2y_d^{pu} y_u^{vs} Q_{quqd}^{(8)vrtu} - \frac{1}{27} g_Y^2 \delta^{pt} Q_{qu}^{(1)uusr} \\
& - \frac{1}{6} g_s^2 \delta^{rs} Q_{qq}^{(1)uptu} - \frac{1}{6} g_s^2 \delta^{rs} Q_{qq}^{(3)uptu} - \frac{8}{27} g_Y^2 \delta^{rs} Q_{qu}^{(1)tpuu} \\
& - \frac{1}{2} y_d^{pu} y_u^{vs} Q_{quqd}^{(1)trvu} - \frac{2}{3} g_s^2 \delta^{rs} Q_{qd}^{(8)tpuu} - \frac{2}{3} g_s^2 \delta^{rs} Q_{qu}^{(8)tpuu} \\
& - \frac{2}{3} \overline{y_d^{tu}} y_d^{pv} Q_{ud}^{(1)sruv} - \frac{2}{3} g_s^2 \delta^{pt} Q_{uu}^{ursu} - \overline{y_u^{ur}} y_u^{pv} Q_{qu}^{(1)tusv} \\
& - \overline{y_u^{tu}} y_u^{vs} Q_{qu}^{(1)vpur} - \frac{4}{3} g_s^2 \delta^{pt} Q_{qu}^{(8)uusr} - \frac{4}{3} g_s^2 \delta^{pt} Q_{ud}^{(8)sruu} \\
& - \frac{3}{2} g_L \overline{y_u^{tr}} \overline{Q_{uW}^{ps}} - \frac{3}{2} g_L y_u^{ps} Q_{uW}^{tr} - \frac{5}{2} g_Y \overline{y_u^{tr}} \overline{Q_{uB}^{ps}} \\
& - \left. \frac{5}{2} g_Y y_u^{ps} Q_{uB}^{tr} - 4\overline{y_d^{tu}} y_d^{pv} Q_{ud}^{(8)sruv} \right]
\end{aligned} \tag{2.44}$$

$$\begin{aligned}
R_{q^c d}^{prst} = & -Q_{qd}^{(1)tpsr} + \frac{1}{16\pi^2} \left[ \frac{1}{9} g_Y^2 \delta^{rs} Q_{qq}^{(1)uutp} + \frac{1}{6} g_Y \overline{y_d^{tr}} \overline{Q_{dB}^{ps}} \right. \\
& + \frac{1}{6} g_Y y_d^{ps} Q_{dB}^{tr} + \frac{2}{9} g_Y^2 \delta^{pt} Q_{dd}^{uusr} + \frac{1}{3} g_Y^2 \delta^{pt} Q_{ld}^{uusr} \\
& + \frac{4}{9} g_Y^2 \delta^{rs} Q_{qu}^{(1)tpuu} + \frac{1}{2} \overline{y_d^{ur}} y_d^{vs} Q_{qq}^{(1)vutp} + \frac{2}{3} g_Y^2 \delta^{pt} Q_{ed}^{uusr} \\
& + \overline{y_d^{ur}} \overline{y_u^{tv}} \left( \overline{Q_{quqd}^{(1)pvus}} - \frac{1}{6} \overline{Q_{quqd}^{(1)uvps}} - \overline{Q_{quqd}^{(8)uvps}} \right) \\
& + \overline{y_d^{tu}} y_d^{pv} Q_{dd}^{uusr} + Q_{Hd}^{sr} \left( 3 \overline{y_d^{tu}} y_d^{pu} - \frac{1}{3} g_Y^2 \delta^{pt} \right. \\
& \left. - 3 \overline{y_u^{tu}} y_u^{pu} \right) + Q_{Hq}^{(1)tp} \left( \frac{1}{3} g_Y^2 \delta^{rs} - 3 \overline{y_d^{ur}} y_d^{us} \right) \\
& + Q_{qd}^{(1)tpsr} \left( -\frac{1}{12} g_Y^2 - \frac{9}{4} g_L^2 \right. \\
& \left. - 8 g_s^2 \right) + y_d^{us} y_u^{pv} Q_{quqd}^{(1)tvur} - \frac{1}{9} g_Y^2 \delta^{pt} Q_{qd}^{(1)uusr} \\
& - \frac{1}{6} y_d^{us} y_u^{pv} Q_{quqd}^{(1)uvtr} - \frac{2}{9} g_Y^2 \delta^{rs} Q_{qd}^{(1)tpuu} - \frac{1}{3} g_Y^2 \delta^{rs} Q_{\ell q}^{(1)uutp} \\
& - \frac{1}{3} \overline{y_d^{ur}} y_d^{pv} Q_{qd}^{(1)tusv} - \frac{1}{3} \overline{y_d^{tu}} y_d^{vs} Q_{qd}^{(1)vpur} - \frac{4}{9} g_Y^2 \delta^{pt} Q_{ud}^{(1)uusr} \\
& - \frac{1}{2} g_L \overline{y_d^{tr}} \overline{Q_{dW}^{ps}} - \frac{1}{2} g_L y_d^{ps} Q_{dW}^{tr} - \frac{2}{3} g_Y^2 \delta^{rs} Q_{qe}^{tpuu} \\
& - y_d^{us} y_u^{pv} Q_{quqd}^{(8)uvtr} - 2 g_s \overline{y_d^{tr}} \overline{Q_{dG}^{ps}} - 2 g_s y_d^{ps} Q_{dG}^{tr} \\
& - 2 \overline{y_d^{ur}} y_d^{pv} Q_{qd}^{(8)tusv} - 2 \overline{y_d^{tu}} y_d^{vs} Q_{qd}^{(8)vpur} - 2 \overline{y_u^{tu}} y_u^{pv} Q_{ud}^{(1)uusr} \\
& \left. - 6 g_s^2 Q_{qd}^{(8)tpsr} \right]
\end{aligned} \tag{2.45}$$

$$\begin{aligned}
R_{q^c d}^{prst} = & -\frac{1}{3} Q_{qd}^{(1)tpsr} - 2 Q_{qd}^{(8)tpsr} + \frac{1}{16\pi^2} \left[ \frac{1}{9} g_Y^2 \delta^{pt} Q_{ld}^{uusr} \right. \\
& + \frac{4}{27} g_Y^2 \delta^{rs} Q_{qu}^{(1)tpuu} + \frac{2}{9} g_Y^2 \delta^{pt} Q_{ed}^{uusr} + \frac{1}{4} \overline{y_d^{ur}} y_d^{vs} Q_{qq}^{(1)vptu} \\
& + \frac{1}{4} \overline{y_d^{ur}} y_d^{vs} Q_{qq}^{(3)vptu} + \frac{1}{3} y_d^{us} y_u^{pv} Q_{quqd}^{(1)tvur} + \frac{1}{2} g_Y \overline{y_d^{tr}} \overline{Q_{dB}^{ps}} \\
& + \frac{1}{2} g_Y y_d^{ps} Q_{dB}^{tr} + \overline{y_d^{ur}} \overline{y_u^{tv}} \left( \frac{1}{3} \overline{Q_{quqd}^{(1)pvus}} + 2 \overline{Q_{quqd}^{(8)pvus}} \right. \\
& \left. - \frac{1}{2} \overline{Q_{quqd}^{(1)uvps}} \right) + \overline{y_d^{tu}} y_d^{pv} Q_{dd}^{ursv} + Q_{dd}^{uusr} \left( \frac{2}{27} g_Y^2 \delta^{pt} \right. \\
& \left. + \frac{2}{9} g_s^2 \delta^{pt} \right) + Q_{Hd}^{sr} \left( \overline{y_d^{tu}} y_d^{pu} - \frac{1}{9} g_Y^2 \delta^{pt} \right. \\
& \left. - \overline{y_u^{tu}} y_u^{pu} \right) + Q_{Hq}^{(1)tp} \left( \frac{1}{9} g_Y^2 \delta^{rs} - \overline{y_d^{ur}} y_d^{us} \right) \\
& + Q_{qd}^{(1)tpsr} \left( -\frac{1}{36} g_Y^2 - \frac{3}{4} g_L^2 \right. \\
& \left. - \frac{16}{3} g_s^2 \right) + Q_{qd}^{(8)tpsr} \left( 4 g_s^2 - \frac{1}{6} g_Y^2 \right. \\
& \left. - \frac{9}{2} g_L^2 \right) + Q_{qq}^{(1)uutp} \left( \frac{1}{27} g_Y^2 \delta^{rs} + \frac{1}{9} g_s^2 \delta^{rs} \right)
\end{aligned} \tag{2.46}$$

$$\begin{aligned}
& + 2y_d^{us} y_u^{pv} Q_{quqd}^{(8)tvur} - \frac{1}{27} g_Y^2 \delta^{pt} Q_{qd}^{(1)uusr} - \frac{2}{27} g_Y^2 \delta^{rs} Q_{qd}^{(1)tpuu} \\
& - \frac{1}{9} g_Y^2 \delta^{rs} Q_{\ell q}^{(1)uutp} - \frac{4}{27} g_Y^2 \delta^{pt} Q_{ud}^{(1)uusr} - \frac{1}{6} g_s^2 \delta^{rs} Q_{qq}^{(1)uptu} \\
& - \frac{1}{6} g_s^2 \delta^{rs} Q_{qq}^{(3)uptu} - \frac{2}{9} g_Y^2 \delta^{rs} Q_{qe}^{tpuu} - \frac{1}{2} y_d^{us} y_u^{pv} Q_{quqd}^{(1)uvtr} \\
& - \frac{2}{3} g_s^2 \delta^{pt} Q_{dd}^{ursu} - \frac{2}{3} g_s^2 \delta^{rs} Q_{qd}^{(8)tpuu} - \frac{2}{3} g_s^2 \delta^{rs} Q_{qu}^{(8)tpuu} \\
& - \frac{2}{3} \overline{y_u^{tu}} y_u^{pv} Q_{ud}^{(1)uusr} - \overline{y_d^{ur}} y_d^{pv} Q_{qd}^{(1)tusv} - \overline{y_d^{tu}} y_d^{vs} Q_{qd}^{(1)vpur} \\
& - \frac{4}{3} g_s^2 \delta^{pt} Q_{qd}^{(8)uusr} - \frac{4}{3} g_s^2 \delta^{pt} Q_{ud}^{(8)uusr} - \frac{3}{2} g_L \overline{y_d^{tr}} \overline{Q_{dW}^{ps}} \\
& - \left[ \frac{3}{2} g_L y_d^{ps} Q_{dW}^{tr} - 4 \overline{y_u^{tu}} y_u^{pv} Q_{ud}^{(8)uvsr} \right]
\end{aligned}$$

$$\begin{aligned}
R_{d^c \ell q^c u}^{prst} = & -2Q_{duq}^{ptsr} + \frac{1}{16\pi^2} \left[ \frac{1}{2} \overline{y_d^{up}} \overline{y_u^{vt}} Q_{qqq}^{svur} + \overline{y_u^{ut}} y_u^{sv} Q_{duq}^{pvur} \right. \\
& + y_e^{ru} y_u^{sv} Q_{duu}^{ptvu} + y_e^{ru} y_u^{sv} Q_{duu}^{pvtu} + \overline{y_d^{up}} \overline{y_u^{vt}} Q_{qqq}^{svur} \\
& \left. + 2\overline{y_d^{up}} y_d^{sv} Q_{duq}^{vtur} - \overline{y_d^{up}} y_e^{rv} Q_{qqu}^{ustv} - 4g_Y^2 Q_{duq}^{ptsr} \right]
\end{aligned} \tag{2.47}$$

$$\begin{aligned}
R_{u^c \ell q^c d}^{prst} = & 2Q_{duq}^{tpsr} + \frac{1}{16\pi^2} \left[ \frac{1}{2} \overline{y_d^{ut}} y_e^{rv} Q_{qqu}^{uspv} + \overline{y_u^{up}} y_u^{sv} Q_{duq}^{tvur} \right. \\
& + y_e^{ru} y_u^{sv} Q_{duu}^{tpvu} - \frac{1}{2} \overline{y_d^{ut}} \overline{y_u^{vp}} Q_{qqq}^{svur} - \overline{y_d^{ut}} y_d^{sv} Q_{duq}^{vpur} \\
& \left. - \overline{y_d^{ut}} \overline{y_u^{vp}} Q_{qqq}^{svur} - 2y_e^{ru} y_u^{sv} Q_{duu}^{tpvu} \right]
\end{aligned} \tag{2.48}$$

$$\begin{aligned}
R_{q^c e u^c q}^{prst} = & 2Q_{qqu}^{tpsr} + \frac{1}{16\pi^2} \left[ \frac{1}{2} \overline{y_e^{ur}} \overline{y_u^{vs}} Q_{qqq}^{vtpu} + \overline{y_e^{ur}} y_d^{pv} Q_{duq}^{vstu} \right. \\
& + Q_{duu}^{usvr} \left( y_d^{pu} y_u^{tv} - y_d^{tu} y_u^{pv} \right) + Q_{duu}^{uvsr} \left( y_d^{pu} y_u^{tv} \right. \\
& + 2y_d^{tu} y_u^{pv} \left. \right) + \overline{y_e^{ur}} \overline{y_u^{vs}} Q_{qqq}^{vptu} - \frac{1}{2} \overline{y_u^{us}} y_u^{pv} Q_{qqu}^{utvr} \\
& \left. - \overline{y_e^{ur}} y_d^{tv} Q_{duq}^{vspu} - \overline{y_u^{us}} y_u^{tv} Q_{qqu}^{upvr} \right]
\end{aligned} \tag{2.49}$$

## References

- [1] B. Grzadkowski, M. Iskrzynski, M. Misiak and J. Rosiek, *Dimension-Six Terms in the Standard Model Lagrangian*, *JHEP* **10** (2010) 085, [[1008.4884](#)].
